# Supplementary material for: Frank-Wolfe with Subsampling Oracle
Source: arXiv:1803.07348 source file (2018-03-20)
Supplement: Supplementary file 1 [file supplementary_and_old_proof.tex]

%This is not a file to compile but just to keep track of the past results
%
%%%%%%%%%%%%%%%%%%%%%%%%%%%%%%%%%%%%%%%%%%%%%%%%%%%%%%%%%%%%%%%%%%%%%%%%%%%%%%%%%%%%%%%%%%%%%%%%%%%%%%%%%%%%%%%%%%%%%%%%%%%%%%%%%%%%%%%%%%%%%%%%%%%%%%%
%%%%%%%%%%%%%%%%%%%%%%%%%%%%%FORMER PROOF OF RFW%%%%%%%%%%%%%%%%%%%%%%%%%%%%%%%%%%%%%%%%%%%%%%%%%%%%%%%%%%%%%%%%%%%%%%%%%%%%%%%%%%%%%%%%%%%%%%%%%%%%%%%
%%%%%%%%%%%%%%%%%%%%%%%%%%%%%%%%%%%%%%%%%%%%%%%%%%%%%%%%%%%%%%%%%%%%%%%%%%%%%%%%%%%%%%%%%%%%%%%%%%%%%%%%%%%%%%%%%%%%%%%%%%%%%%%%%%%%%%%%%%%%%%%%%%%%%%%
\begin{theorem}\label{th:expectation_rate}
Consider Algorithm \ref{algo:Randomized_FW_general} on $\mathcal{M}=\text{Conv}(\mathcal{V})$ with random sub-sampling of size $p$. After $t$ iterations:
\begin{eqnarray}
\mathbb{E}(f(\xx_t))-f(\xx^*) \leq \frac{|\mathcal{V}|^2}{p^2} \frac{2C_f}{t+2},
\end{eqnarray}
where $C_f$ stands for the curvature constant defined as
\begin{eqnarray*}
C_f\coloneqq \underset{\substack{x,s\in\mathcal{M},\gamma\in [0,1] \\ y=x+\gamma (s-x)}}{\text{sup }} {\frac{2}{\gamma^2}\big( f(y)-f(x)-\langle\nabla f(x),y-x\rangle \big)}.
\end{eqnarray*}
\end{theorem}

\begin{proof}
Note $r_t=-\nabla f(\xx_t)$. Denote by $\tilde{\ss}_t$ and $\ss_t$ the FW vertex and the Randomized FW vertex at iteration $t$. Similarly denote by $\tilde{g}_t=\langle\tilde{\ss}_t-\xx_t;r_t \rangle$ the FW dual gap and by $g_t=\langle \ss_t-\xx_t;r_t \rangle$ the corresponding partial randomized dual gap.
For an update $\xx_{t+1}(\gamma)=\xx_t+\gamma (\ss_t-\xx_t)$ we have:
\begin{eqnarray}\label{eq:descent_lemma}
f(\xx_{t+1})\leq f(\xx_{t+1}(\gamma))&\leq f(\xx_{t}) -\gamma \langle \ss_t-\xx_t;r_t \rangle\nonumber\\
&\qquad+\frac{\gamma^2}{2} C_f~~\forall \gamma\in [0;1]~,
\end{eqnarray}
where the first inequality comes from the line search and the second one from the definition of the curvature constant {\blue FP: need to be made precise what inequalities are used}.


Eq. \eqref{eq:descent_lemma} is valid for any $\gamma\in[0,1]$. In particular, for $\gamma \mathds{1}\{ g_t \geq 0\}$ and any $\gamma\in[0,1]$:
\begin{eqnarray}\label{eq:descent_lemma_modified_gamma}
f(\xx_{t+1})\leq f(\xx_{t}) -\gamma \mathds{1}\{ g_t \geq 0\} g_t +\mathds{1}\{ g_t \geq 0\} \frac{\gamma^2}{2} C_f
\end{eqnarray}
With $\mathbf{E}$ (resp. $\mathcal{P}$) the expectation (resp. the probability) with respect to the $t$ sub-sampling, conditionally on whole past:
\begin{eqnarray}\label{eq:expectation}
\mathbf{E} \left( f(\xx_{t+1}) \right)\leq f(\xx_{t}) - \gamma \mathbf{E} \left( 1_{ g_t \geq 0} g_t \right) +\mathcal{P}_t(g_t \geq 0) \frac{\gamma^2}{2} C_f.
\end{eqnarray}

We will now bound the two expectation terms in the right hand side. 
When $s_t=\tilde{s}_t$, $g_t=\tilde{g}_t$.
Because $1_{ g_t \geq 0} g_t $ is positive:
\begin{eqnarray}\label{eq:key_analysis}
\mathbf{E} \left( 1_{ g_t \geq 0} g_t \right) \geq \mathcal{P}_t(s_t=\tilde{s}_t) \tilde{g}_t,
\end{eqnarray}
which leads to\footnote{We upper-bound grossly $\mathcal{P}_t(g_t \geq 0)$ by $1$ because a tighter bound requires knowledge on the gradient and the geometry of the polytope.}:
\begin{eqnarray*}
\mathbf{E}\left( f(\xx_{t+1}) \right)\leq f(\xx_{k}) - \gamma \mathcal{P}_t(g_t=\tilde{g}_k) \tilde{g}_k  + \frac{\gamma^2}{2} C_f,
\end{eqnarray*}
$\tilde{g}_t$ is the FW dual gap from the classical algorithm and as such an upper bound of $h(\xx_t)=f(\xx_t)-f(\xx^*)$: 
\begin{eqnarray*}
\mathbf{E}\left( h(\xx_{t+1}) \right)\leq (1 - \gamma \mathcal{P}(g_t=\tilde{g}_t))  h(\xx_{t}) +\mathcal{P}_t(g_t \geq 0) \frac{\gamma^2}{2} C_f,
\end{eqnarray*}
Finally $\mathcal{P}_t(s_t=\tilde{s}_t) \geq \frac{p}{|\mathcal{V}|}$. Indeed the respective definition of $\tilde{s}_t$ and $s_t$ are: {\blue This is not trivial and depends crucially on the sampling scheme. Please explain} 
\begin{eqnarray}
\ss_t\in\underset{s\in \mathcal{V}_p}{\argmin} \langle s,\nabla f(\xx_{t})\rangle\\
\tilde{\ss}_t\in\underset{s\in \mathcal{V}}{\argmin} \langle s,\nabla f(\xx_{t})\rangle
\end{eqnarray}
Name by $\mathcal{H}=\{s\in\mathcal{V}~|~\langle s,\nabla f(x_t)\rangle= \langle \tilde{s}_t,\nabla f(x_t)\rangle \}$. The probability $\mathcal{P}_t(s_t=\tilde{s}_t)$ is about counting the number of subset of $\mathcal{V}$ of size $p$ containing an element of $\mathcal{H}$. The worth case being when $\mathcal{H}$ is a singleton:
\begin{eqnarray*}
\mathcal{P}_t(s_t=\tilde{s}_t)\geq \frac{{{|\mathcal{V}|}\choose{p-1}}}{{{|\mathcal{V}|}\choose{p}}}=\frac{p}{|\mathcal{V}|}
\end{eqnarray*}

We thus have:
\begin{eqnarray*}
\mathbf{E}\left( h(\xx_{t+1}) \right)\leq (1 - \gamma \frac{p}{|\mathcal{V}|})  h(\xx_{t}) + \frac{\gamma^2}{2} C_f.
\end{eqnarray*}
Considering lately a pre-determined choice of $\gamma$ at each iteration, because $\mathbb{E}(h(\xx_{t+1}))=\mathbb{E}(\mathbf{E}(h(\xx_{t+1})))$, it has to be that:
\begin{eqnarray}\label{eq:recursion_inequality}
\mathbb{E}\left( h(\xx_{t+1}) \right)\leq (1 - \gamma \frac{p}{|\mathcal{V}|})  \mathbb{E}\left(h(\xx_{t})\right) + \frac{\gamma^2}{2} C_f.
\end{eqnarray}

It is then just a matter of recursion to get the final bound. Using \citep[Th. 1]{jaggi2013revisiting} , we know that for $\gamma=\frac{2}{t+2}$ and:
\begin{eqnarray*}
h_{t+1}\leq (1-\gamma)h_t+\frac{\gamma^2}{2}C_f,
\end{eqnarray*}
by induction {\blue you will need to explain this induction scheme (you cannot assume that the reviewer knows the Jaggi proof). Furthermore, the use of expectations requires a bit of work to be rigorous on how to obtain full expectations from conditional expectations.} there is:
\begin{eqnarray*}
h_t\leq \frac{2C_f}{t+2}.
\end{eqnarray*}
In our case with $\gamma=\frac{|\mathcal{V}|}{p}\frac{2}{k+2}$, we get {\blue FP: careful, in the algorithm you are using exclusively line search. Careful2: this can be greater than 1}:
\begin{eqnarray}
\mathbb{E}(f(\xx_t))-f(\xx^*) \leq \frac{|\mathcal{V}|^2}{p^2} \frac{2C_f}{t+2}
\end{eqnarray}

\end{proof}


%%%%%%%%%%%%%%%%%%%%%%%%%%%%%%%%%%%%%%%%%%%%%%%%%%%%%%%%%%%%%%%%%%%%%%%%%%%%%%%%%%%%%%%%%%%%%%%%%%%%%%%%%%%%%%%%%%%%%%%%%%%%%%%%%%%%%%%%%%%%%%%%%%%%%%%
%%%%%%%%%%%%%%%%%%%%%%%%%%%%%PROOF IN PROBABILITY%%%%%%%%%%%%%%%%%%%%%%%%%%%%%%%%%%%%%%%%%%%%%%%%%%%%%%%%%%%%%%%%%%%%%%%%%%%%%%%%%%%%%%%%%%%%%%%%%%%%%%
%%%%%%%%%%%%%%%%%%%%%%%%%%%%%%%%%%%%%%%%%%%%%%%%%%%%%%%%%%%%%%%%%%%%%%%%%%%%%%%%%%%%%%%%%%%%%%%%%%%%%%%%%%%%%%%%%%%%%%%%%%%%%%%%%%%%%%%%%%%%%%%%%%%%%%%

\subsection{Beyond expectation convergence results}
% Say that stochastic is a term cast for stochastic gradient, we follow Frandi is the Randomized term which is no a block coordinate descent algorithm because there is no separable domain structure.

In many stochastic scenario of Frank-Wolfe the proofs are provided in expectation (\cite{Frandi2016} or \cite{hazan2016variance}). The study of the variance of $h(\xx_t)$ is often jilted but also weaker than observed experiments which suggest that the rate of convergence in expectation holds in a deterministic manner. Here we propose a theoretical analysis of algorithm \ref{algo:Randomized_FW_general} that allows a convergence guarantee with a given high probability.


Theorem \ref{th:proba_convergence} address this concern by quantifying how many times the direction given by the randomized oracle would match the FW oracle (see lemma \ref{lem:prob_k_among_K}). Then lemma \ref{lem:analysis_k_among_K} express the decrease of the function after K iterates of Randomized FW when doing at least $k$ FW classical updates.

Theorem \ref{th:RFW_variance_analysis} uses this analysis to prove a $\mathcal{O}(\frac{1}{K})$ rate for the variance of $h(\xx_t)$.
 
Although the proved rate in theorem \ref{th:expectation_rate} is $\mathcal{O}(\frac{1}{K})$, it is a conservative result in the sens that to obtain a given precision, classical Frank-Wolfe would theoretically required less basic operations compared to its randomized counter-part. To obtained better constants rates, we would like to analyze the impact of a step that does not match with the FW classical one. This heavily relies on the sequence $(\langle - \nabla f(\xx_t); v \rangle)_{v\in\mathcal{V}}$ and thus requires additional assumptions on the polyhedral domain and the gradient. 

{\color{red}{try to finish that}}Theorem \ref{th:deterministic_error_proof} tries to address this issue with a bound accounting for all the improvement of the various iterate of Randomized FW. It is descriptive by nature, e.g. it does not lead to a practical implementation in the algorithm, because it requires a general assumption over the gradient.

%analysis of the decreasing when k steps are matching with the classical FW direction
\begin{lemma}\label{lem:analysis_k_among_K}
Consider any initial condition $\xx_0$, and $\xx_{K}$ the iterate of the Randomized Frank-Wolfe. Assume that among the $K$ iteration there have been at least $k$ sub-sample oracle that gave the same direction as the Frank-Wolfe linear oracle. We then have:
\begin{align}\label{eq:converg_k_among_K}
h(\xx_{K+1})=f(\xx_{K+1})-f(\xx^*) \leq  \frac{2C_f}{k+3}
\end{align}
\end{lemma}

\begin{proof}
Let's make the proof by induction with the help of deterministic results from \cite{jaggi_revisiting_2013} Theorem 1 and lemma 5. We want to show by induction on $K\geq 1$, the following property:
\begin{align}
\mathcal{P}_{K}: \forall k\in\{1;\cdots;K\},~\forall \xx_0:\nonumber\\
h(\xx_{K+1})\leq \frac{2C_f}{k+3},\label{eq:condition_P}
\end{align}
where $k$ is the number of classic Frank-Wolfe steps among the $K$ iterations of the Randomized Frank-Wolfe.\\

Initialization: $\mathcal{P}_1$ follows from Theorem 5. in \cite{jaggi_revisiting_2013}.

Heredity: Let $\mathcal{P}_{K_0}$ to be true. Consider a $\xx_0$ and a corresponding sequence $(\xx_{i})_{0\leq i\leq K_0+2}$, realization of the Randomized FW algorithm. If $k=K_{0}+1$, again (\ref{eq:condition_P}) is an application of Theorem 5.\\

For $k\leq K_{0}+1$, let's distinguish between two cases.

If the $K_0+1$-ith iteration is not a classical Frank-Wolfe step, it means that all the $k$ classical Frank-Wolfe step were realized before $K_0$. We can thus apply $\mathcal{P}_{K_0}$ to get:
\begin{align*}
h(\xx_{K_0+1})\leq \frac{2C_f}{k+3}.
\end{align*}
Finally by exact line-search we have $h(\xx_{K_0+2})\leq h(\xx_{K_0+1})$, so that:
\begin{align}
h(\xx_{K_0+2})\leq \frac{2C_f}{k+3},
\end{align}
which proves $\mathcal{P}_{K_0}$.

If the $K_0+1$-ith iteration is a classical Frank-Wolfe step. We can now apply $\mathcal{P}_{K_0}$ to $k-1$ to get:
\begin{align*}
h(\xx_{K_0+1})\leq \frac{2C_f}{k+2}.
\end{align*}
Then from lemma 5 in \cite{jaggi_revisiting_2013} we have:
\begin{align*}
h(\xx_{K_0+2}(\gamma))\leq (1-\gamma)h(\xx_{K_0+1})+\gamma^2 \frac{C_f}{2},
\end{align*}
where $\gamma\in [0;1]$. Since $\xx_{i}=\xx_{i}(\gamma_{\text{optimal}})$, we have that for all $\gamma\in [0;1]$, $h(\xx_{K_0+2})\leq h(\xx_{K_0+2}(\gamma))$. By $\gamma=\frac{2}{k+2}$, we obtain that:
\begin{eqnarray*}
h(\xx_{K_0+2}) &\leq & (1-\frac{2}{k+2})\frac{2C_f}{k+2}+\frac{2C_f}{(k+2)^2}\\
h(\xx_{K_0+2}) &\leq & \frac{2C_f}{k+3}
\end{eqnarray*}
Property $\mathcal{P}_{K_0+1}$ is then proved. 
\end{proof}


%analysis of the proba of F_k
\begin{lemma}\label{lem:prob_k_among_K}
Denote by $F_K$ the random variable that counts the number of iterate among $K$ consecutive ones of algorithm \ref{algo:Randomized_FW_general} in which the direction given by the sub-sampled linear oracle is the one given by the linear oracle:
\begin{eqnarray}
\mathbb{P}(F_K\leq k)\leq \mathbb{P}(B\leq k),
\end{eqnarray}
where $B$ is a binomial $\mathcal{B}(K,\frac{p}{|\mathcal{V}|})$ where $p$ is the size of the random batch on which the sub-sample oracle is performed.
\end{lemma}

\begin{proof}
At the $i$-th iteration of Randomized Frank-Wolfe, the direction $v_i$ of the sub-sampled linear oracle is such that:
\begin{equation}\label{eq:sub_sample_linear_oracle}
    v_i\in\underset{v\in \mathcal{V}_p}{\argmin} \langle v,\nabla f(\xx_{i-1})\rangle
\end{equation}
where $\mathcal{V}_p$ is a random subset of size $p$ of the set of vertex $\mathcal{V}$. The direction $v_i^*$ from the linear oracle is such that:
\begin{equation}\label{eq:linear_oracle}
    v_i^*\in\underset{v\in \mathcal{V}}{\argmin} \langle v,\nabla f(\xx_{i-1})\rangle.
\end{equation}

At an iterate $\xx_i$ it is the less likely case for the sub-sampled oracle to output the linear oracle direction when all the values of $(\langle v,\nabla f(\xx_{i-1})\rangle)_{v\in\mathcal{V}}$ are distinct. Indeed if they are not, denote by $s^{\prime}$ the cardinal of the sequence, then with probability $p(s^{\prime})=\mathbb{P}(\underset{i\in [1;\cdots;s^{\prime}]_p}{\min i}=1)$, we have $v_i=v_i^*$. And $p(s^{\prime})\leq p(s)$. It implies that the cumulative distribution of $F_K$ is upper bounded by that of $B\sim Bin(K,p(s))$ when each iterate is this situation.

\end{proof}



%general theorem
\begin{theorem}\label{th:proba_convergence}
With probability $1-\frac{p_1}{K}$, doing $K$ iterations of the Randomized FW leads to:
\begin{eqnarray}\label{eq:proba_rate}
f(\xx_{K+1})-f(\xx^*)\leq \frac{2C_f}{\frac{K}{p_1}+3},
\end{eqnarray}
with $p_1=\frac{5}{2p_0}+\sqrt{\frac{1-p_0}{p_0}}$, where $p_0=\frac{p}{s}$.
\end{theorem}



\begin{proof}
Consider a number of iteration $K$ and a small probability $\alpha$. We first would like to control the quantity:
\begin{eqnarray}
\mathbb{P}(F_{K}\geq k) \geq 1-\alpha
\end{eqnarray}
We have probabilistic information on $F_{K}$. Indeed with lemma \ref{lem:prob_k_among_K} for $B\sim\mathcal{B}(K,\frac{p}{s})$:
\begin{eqnarray}\label{eq:proba_bound_F}
\mathbb{P}(F_K \leq k)\leq \mathbb{P}(B \leq k)
\end{eqnarray}
With $p_0=\frac{p}{s}$, from \cite{feller1} and for any $K\geq \frac{k}{p_0}$:
\begin{eqnarray}\label{eq:feller}
\mathbb{P}(B\leq k)\leq \frac{(K-k)p_0}{(Kp_0-k)^2}
\end{eqnarray}

Let's denote by $K_{\alpha}$ the smallest $K\geq \frac{k}{p_0}$ such that $\frac{(K-k)p_0}{(Kp_0-k)^2}\leq \alpha$, combining (\ref{eq:feller}) with (\ref{eq:proba_bound_F}), we have that for $K\geq K_{\alpha}$ with probability at least $1-\alpha$:
\begin{eqnarray}\label{eq:key_inequality}
f(\xx_{K+1})-f(\xx^*)\leq \frac{2C_f}{k+3}.
\end{eqnarray}

%form of K_alpha
Let's now find an analytic form of $K_{\alpha}$. It satisfies :
\begin{align*}
\alpha \alpha p_0^2 K_{\alpha} -(2\alpha k + 1)p_0 K_{\alpha} + \alpha k^2 +k p_O \geq 0.
\end{align*}
Let's denote by $P(K)$ the polynomial in the left hand side and $\xx_+$ its greatest root if he has one, $0$ otherwise. Then:
 \begin{eqnarray}
 K_{\alpha}=\max\{ \frac{k}{p_0} , \xx_+\}
 \end{eqnarray}
 The discriminant of $P(K)$ is:
 \begin{eqnarray}
 \Delta =p_0^2 [4\alpha k(1-p_0)+1],
 \end{eqnarray}
and $\xx_+$ satisfies:
\begin{eqnarray}
\xx_+=\frac{k}{p_0}+\frac{1+2\sqrt{\alpha k (1-p_0)+1}}{2 \alpha p_0}\\
\xx_+\leq \frac{k}{p_0}+\frac{3}{2\alpha p_0}+\sqrt{\frac{k}{\alpha}}\sqrt{\frac{1-p_0}{p_0}}=H(k,\alpha).
\end{eqnarray}
It follows that any $K\geq \xx_+$ would be a good choice for $K_{\alpha}$. Given $k$ let's consider $\alpha_k=\frac{1}{k}$, we have that $H(k,\alpha_k)=k p_1$ with $p_1=\frac{1}{p_0}+\frac{3}{2p_0}+\sqrt{\frac{1-p_0}{p_0}}$. Finally using (\ref{eq:key_inequality}),we have that for any $k\geq 1$, with probability $1-\frac{1}{k}$, for any $K\geq k p_1$:
\begin{eqnarray}
f(\xx_{K+1})-f(\xx_*)\leq \frac{2 C_f}{k+3}.
\end{eqnarray}
In particular for a $K\geq \lfloor p_1 \rfloor$, with probability $1-\frac{p_1}{K}$:
\begin{eqnarray}
f(\xx_{K+1})-f(\xx_*)\leq \frac{2 C_f}{\frac{K}{p_1}+3}.
\end{eqnarray}


\end{proof}


%result in variance
Theorem \ref{th:proba_convergence} allows to give a bound on the variance of $h(\xx_t)$:
\begin{theorem}\label{th:RFW_variance_analysis}
After K>0 iterations of algorithm \ref{algo:Randomized_FW_general}:
\begin{eqnarray}\label{eq:variance_result_RFW}
\text{Var}(f(\xx_k)-f(\xx^*))\leq p_1\frac{(2C_f+\mathcal{D})}{K}
\end{eqnarray}
with $p_1=\frac{5}{2p_0}+\sqrt{\frac{1-p_0}{p_0}}$, where $p_0=\frac{p}{s}$. $\mathcal{D}$ is the diameter of $\mathcal{M}$.
\end{theorem}

\begin{proof}
From theorem \ref{th:deterministic_error_proof}, we have that with probability $1-\frac{p_1}{K}$, $h(\xx_{K+1})=f(\xx_{K+1})-f(\xx^*)$ satisfies eq. (\ref{eq:proba_rate}). Otherwise we bound $h(\xx_{K+1})$ by the diameter $\mathcal{D}$ of the polytope $\mathcal{M}$. Denote by $\mathbf{V}_{K+1}$, the variance of $h(\xx_{K+1})$, it leads to:
\begin{eqnarray*}
\mathbf{V}_{K+1}\leq (1-\frac{p_1}{K})\frac{2C_f}{\frac{K}{p_1}+3} +\frac{p_1}{K}\mathcal{D}.
\end{eqnarray*}
Essentially the rate will be in $\mathcal{O}(\frac{1}{K})$ so that we can gave away the $(1-\frac{p_1}{K})$:
\begin{eqnarray*}
\mathbf{V}_{K+1}\leq \frac{2C_f}{\frac{K}{p_1}+3} +\frac{p_1}{K}\mathcal{D}\\
\mathbf{V}_{K+1}\leq p_1\frac{2C_f+\mathcal{D}}{K}
\end{eqnarray*}
\end{proof}


%WITH ASSUMPTION ON THE GRADIENT
Although theorem \ref{th:proba_convergence} provides the same expectation rate of (\ref{eq:expectation_rate}) but in high probability, the analysis throw away the decrease of the iterates that do not match with the deterministic FW direction. In theorem \ref{th:deterministic_error_proof} we specialize to the $\ell_1$ ball in which the difference between linear oracle and the sub-sampled linear oracle can be easily expressed. We provided bounds based on the convergence analysis of \cite{freund2016new}.

\begin{theorem}\label{th:deterministic_error_proof}
After $K$ iterations of algorithm  (\ref{algo:Randomized_FW_general}) of the $\ell_1$-ball in $\mathbb{R}^s$, with a random sub-sample of size $p$, we have for $h(\xx_{K})=f(\xx_{K})-f(\xx^*)$ :
\begin{align}\label{eq:general_deterministic_bound}
h(\xx_{K})\leq \frac{4.5 C_f}{k+4}+\frac{\sum_{i=1}^K{\gamma_i \delta_i}}{\sum_{i=1}^K{\gamma_i}},
\end{align}
where $s_{r}^i\in\underset{j\in\mathcal{I}_p}{\argmax} |\nabla f(\xx_{i-1})|_j$, $\gamma_i$ the exact step-size and $\delta_i=(|\nabla f(\xx_{i-1})|_{(s)}-|\nabla f(\xx_{i-1})|_{(s_{p}^i)})$. By adding an hypothesis on the distribution of the gradient of the form:
\begin{eqnarray}
to complete
\end{eqnarray}
we have the following guarantee of convergence:
\begin{eqnarray}
to complete
\end{eqnarray}

\end{theorem}

\begin{proof}
To the prove this theorem we make an extensive use of results from \cite{freund2016new}. Indeed we apply Theorem $5.1$, where the part of the upper-bound that does not depend
on $\delta_t$ is exactly that of Theorem $2.2$ on which is applied Bound $3.1$ ($G_k$ corresponds to the FW dual certificate to which we do not have access):
\begin{eqnarray}\label{eq:bound_freund}
\underset{i=1;\cdots;K}{G_i}\leq \frac{4.5 C_f}{k+4}+\frac{\sum_{i=1}^K{\bar{\alpha}_i \delta_i}}{\sum_{j=1}^{K}{\bar{\alpha}_i}},
\end{eqnarray}
where $\bar{\alpha}_i$ are any chosen step-size and $\delta_i$, the error between the linear oracle and its randomized counter-part.

When choosing exact step size $\gamma_i$, it ensures decrease of the dual gap at each iteration so that:
\begin{eqnarray}\label{decrease of the dual gap}
g(\xx_{K})=\underset{i=1;\cdots;K}{\min}{g(\xx_i)}\leq \underset{i=1;\cdots;K}{\min}{G_i}.
\end{eqnarray}
Besides from algorithm \ref{algo:Randomized_FW_general}, the decrease we have:
\begin{eqnarray}
\delta_i=(|\nabla f(\xx_{i-1})|_{(s)}-|\nabla f(\xx_{i-1})|_{(s_{p}^i)}),
\end{eqnarray}
from which \ref{eq:general_deterministic_bound} follows.

We see that the error will depend on how the coefficients  $(|\nabla f(\xx)|_i)_{i}$ of the gradient spread. We propose the following form of assumption over the gradient:
\begin{eqnarray}\label{eq:assumption_gradient}
|\nabla f(\xx)|_{(i)}\geq |\nabla f(\xx)|_{(d)} \frac{\exp(i \lambda_x)-1}{\exp(d\lambda_x)-1},
\end{eqnarray}
where $d$ is the dimension on which we naturally consider the $\ell_1$-ball.
\end{proof}


%%%%%%%%%%%%%%%%%%%%%%%%%%%%%%%%%%%%%%%%%%%%%%%%%%%%%%%%%%%%%%%%%%%%%%%%%%%%%%%%%%%%%%%%%%%%%%%%%%%%%%%%%%%%%%%%%%%%%%%%%%%%%%%%%%%%%%%%%%%%%%%%%%%%%%%
%%%%%%%%%%%%%%%%%%%%%%%%%%%%%OLD PROOF RAFW%%%%%%%%%%%%%%%%%%%%%%%%%%%%%%%%%%%%%%%%%%%%%%%%%%%%%%%%%%%%%%%%%%%%%%%%%%%%%%%%%%%%%%%%%%%%%%%%%%%%%%
%%%%%%%%%%%%%%%%%%%%%%%%%%%%%%%%%%%%%%%%%%%%%%%%%%%%%%%%%%%%%%%%%%%%%%%%%%%%%%%%%%%%%%%%%%%%%%%%%%%%%%%%%%%%%%%%%%%%%%%%%%%%%%%%%%%%%%%%%%%%%%%%%%%%%%%



% One important point is to distinguish between $\gamma_{\text{max}}$ and $\widetilde\gamma_{\text{max}}$ for the greatest admissible step size along direction $\widetilde\dd_t$ for Classical Away Step or $\dd_t$ for Randomized Away Step:
% \begin{eqnarray}\label{eq:gamma_max_randomized}
% \gamma_{\text{max}} = \left\{
%     \begin{array}{ll}
%         1 & \text{if} \langle - \nabla f(\xx_t);\dd_t^{\text{FW}}\rangle \geq \langle - \nabla f(\xx_t);\dd_t^A\rangle  \\
%         \frac{\alpha_{v_t}}{1-\alpha_{v_t}} & \text{if} \langle - \nabla f(\xx_t);\dd_t^{\text{FW}}\rangle < \langle - \nabla f(\xx_t);\dd_t^A\rangle 
%     \end{array}
% \right.
% \end{eqnarray}
% while:
% \begin{eqnarray}\label{eq:gamma_max_classical}
% \widetilde{\gamma}_{\text{max}} = \left\{
%     \begin{array}{ll}
%         1 & \text{if} \langle-\nabla f(\xx_t);\widetilde\dd_t^{\text{FW}}\rangle \geq \langle-\nabla f(\xx_t);\dd_t^A\rangle  \\
%         \frac{\alpha_{v_t}}{1-\alpha_{v_t}} & \text{if} \langle-\nabla f(\xx_t);\widetilde\dd_t^{\text{FW}}\rangle < \langle-\nabla f(\xx_t);\dd_t^A\rangle 
%     \end{array}
% \right.
% \end{eqnarray}
% where we note that given $\xx_t$ the away direction $\dd^A$ is the same in both version.
%Since we always have $\langle-\nabla f(\xx_t);\dd_t^{FW}\rangle \geq \langle-\nabla f(\xx_t);\widetilde\dd_t^{FW}\rangle$, the Randomized Away FW have a tendency to favor more Away-steps more than its deterministic counter-part.


\begin{proof}
The proof roughly follows that of Theorem 8 in  \cite{lacoste2015global}. 

\textit{Upper bounding $h_t$}: Considering an iterate $\xx_{t}$ that is not optimal (i.e., $\xx_t \neq \xx^*$) we have:
\begin{eqnarray}\label{eq:upper_bound_h}
f(\xx_{t})-f(\xx^*)=h_t\leq \frac{\widetilde g_t^2}{2\mu_f^{A}},
\end{eqnarray}
where $\widetilde g_t$ is the pair-wise dual gap\footnote{It is an upper bound on the dual gap. Indeed:
\begin{eqnarray}
v_t\in\underset{v\in\mathcal{S}_t}{\argmin } {\langle r_t;v\rangle},
\end{eqnarray} 
so that:
\begin{eqnarray}
g_t^{PW}=\langle s_t;r_t\rangle-\underset{v\in\text{Conv}(\mathcal{S}_t)}{\min } {\langle r_t;v\rangle}.
\end{eqnarray}
Finally since $\xx_t\in\text{Conv}(\mathcal{S}_t)$, we have that:
\begin{eqnarray}
g_t^{PW}\geq \langle s_t-\xx_t;r_t\rangle.
\end{eqnarray}
The right side argument being the FW dual gap, the Pair-Wise dual gap, is an upper bound on the dual gap.
}, e.g. $\widetilde g_t=\langle \widetilde\ss_t-\vv_t;-\nabla f(\xx_t)\rangle$.  $\widetilde\ss_t$ and $\vv_t$ are respectively the FW vertex and the away vertex in the classical Away step algorithm (note that the away vertex of the randomized variant does not depend on $\mathcal{V}_t$ and so coincides with the away vertex of the non-randomized variant). We will later relate this to the partial pair-wise dual gap $g_t$, where the FW vertex $\widetilde s_t$ has been replaced by the randomized FW vertex $s_t$ coming from the sub-sampled oracle.

This results is the same as in \citep[Eq. (28)]{lacoste2015global} because it only comes from the definition of the affine invariant version of the strong convexity parameter.\\

\textit{Lower bounding progress $h_t-h_{t+1}$}:

The idea is to get away with the randomness and do the same type of cases distinction of \cite{lacoste2015global} or \cite{beck2013convergence}.

By definition of the curvature constant we have the following inequality, with $\xx_{t, \gamma} \stackrel{\text{def}}{=}\xx_{t}+\gamma \dd_{t}$:
\begin{eqnarray}\label{eq:curvature_constant_away}
f(\xx_{t, \gamma})\leq f(\xx_{t})+\gamma \langle\nabla f(\xx_{t});\dd_{t}\rangle+\frac{\gamma^2}{2}C_f.
\end{eqnarray}
We denote by $\gamma_t^{*}$\footnote{Conditionally on $\xx_t$, it is a random variable with respect to the $t^{ith}$ sub-sampling.} the step-size from exact line-search at iteration $t$, e.g. which satisfies:
\begin{eqnarray}
\gamma_t^{*}\in\underset{\gamma\in[0,\gamma_{\text{max}}]}{\argmin} f(\xx_{t}+\gamma \dd_t)=F(\gamma).
\end{eqnarray}
Precisely in RAFW, $\xx_{t+1}=\xx_{t, \gamma_t^{*}}$. Using the curvature constant definition we have:
\begin{align}
f(\xx_{t+1})\leq f(\xx_{t, \gamma})&\leq f(\xx_{t})+\gamma \langle\nabla f(\xx_{t});\dd_{t}\rangle\nonumber\\
&\qquad+\frac{\gamma^2}{2}C_f ~~\forall \gamma\in [0;\gamma_{\text{max}}]~.
\end{align}

Using lemma \ref{lem:progress_direction_sub_away} we get for all $\gamma\in[0;\gamma_{\text{max}}]$:
\begin{align}\label{eq:lower_bound_h}
f(\xx_{t+1})&\leq f(\xx_{t})-\gamma \frac{g_t}{2}+\frac{\gamma^2}{2}C_f\nonumber\\
\gamma \frac{g_t}{2}-\frac{\gamma^2}{2}C_f&\leq f(\xx_{t})-f(\xx_{t+1})
\end{align}

The left hand side of (\ref{eq:lower_bound_h}) is maximized for $\gamma_t^B=\frac{g_t}{2C_f^A}\geq 0$ (the positiveness comes from lemma \ref{lem:progress_direction_sub_away}). Let's distinguish between the cases.


\textbf{Cases $\gamma_{\text{max}}\geq 1$}. These situations does not necessarily involve the choice of a Frank-Wolfe step but ensure that when choosing an away-step, there is enough mass on the away vertex $\vv_t$ to allow an important decrease of the objective function. Let's distinguish whether $\gamma^B_t$ is admissible or not.

\indent\textbf{case $\gamma_t^B\leq \gamma_{\text{max}}$:} Evaluating (\ref{eq:lower_bound_h}) on $\gamma=\gamma_t^B$ we get:
\begin{eqnarray}
h_t(\xx_t) -  h(\xx_{t+1}) \geq \frac{g_t^2}{8 C_f^A}
\end{eqnarray}
We now take the expectation with respect to the $t$-ith sub-sampling conditionally of $\xx_t$ and on the random event $C_1=\{\gamma_t^B\leq \gamma_{\text{max}}~~\gamma_{\text{max}}\geq 1\}$:
\begin{eqnarray}
h_t -  \textbf{E}_t \big(h(\xx^{(t+1)})\big) \geq \frac{\textbf{E}_t \big(g_t^2\big)}{8 C_f^A}.
\end{eqnarray}
With probability greater than $p_0=\frac{p}{|\mathcal{V}|}$, $\ss_t=\tilde{\ss}_t$ and thus $g_t=\widetilde g_t$ from which follows:
\begin{eqnarray}\label{eq:lower_bound_expectation}
h_t - \textbf{E}_t \big(h_{t+1}\big) \geq p_0 \frac{\tilde{g}_t^2}{8 C_f^A}.
\end{eqnarray}


{\red TK: Here there is a huge problem that I don't know how to overcome. Indeed the expectation is conditionally on $\xx_t$ and on the random event that $\gamma_{\text{max}}\geq 1$. The issue is that when doing an away step (e.g. $\gamma_{\text{max}} > 1$, a sub-event of our random event ), it means that:
\begin{eqnarray}
\langle r_t;d_t^A\rangle \geq \langle r_t;d_t^{FW}\rangle
\end{eqnarray}
But $\xx_t$ is known and so is $\langle r_t;d_t^A\rangle $ and $\langle r_t;\tilde{d}_t^{FW}\rangle$. It then follows that if $\langle r_t;\tilde{d}_t^{FW}\rangle>\langle r_t;d_t^A\rangle$, \textbf{the probability for $\tilde{s}_t$ to be equal to $s_t$ is zero} and so the previous lower bound fails to be true... 

}


Combined with \eqref{eq:upper_bound_h}, we have:
\begin{eqnarray}
h_t - \mathbf{E}_t\big( h_{t+1}\big) \geq \frac{p_0 \mu_f^A}{4 C_f^A} h_t\\
\mathbf{E}_t\big( h_{t+1} \big) \leq (1- \frac{p_0  \mu_f^A}{4 C_f^A}) h_t
\end{eqnarray}


\indent\textbf{case $\gamma_t^B\geq \gamma_{\text{max}}$:} We then have that $\frac{g_t}{2}\geq C_f^A$ so that 
\eqref{eq:lower_bound_h} transforms into (for $\gamma\in[0,\gamma_{\text{max}}]$):
\begin{align}
f(\xx_{t})-f(\xx_{t+1}) &\geq \frac{g_t}{2}(\gamma -\frac{\gamma^2}{2}),
\end{align}
which leads when applied for $\gamma=1$:
\begin{align}
f(\xx_{t})-f(\xx_{t+1}) &\geq \frac{g_t}{4}.
\end{align}
Again, applying the expectation $\mathbf{E}_t$ (which is conditionally on knowing $\xx_t$ and $C_2=\{\gamma_t^B\geq \gamma_{\text{max}}~;\gamma_{\text{max}}\geq 1~\}$) and its lower bound, we get:
\begin{align}
f(\xx_{t})-\mathbf{E}_t\big(f(\xx_{t+1})\big) &\geq p_0\frac{\tilde{g}_t}{4}.
\end{align}
Being the pair-wise dual gap, $\tilde{g}_t$ is an upper bound on $h(\xx_t)$. We get:
\begin{align}
f(\xx_{t})-\mathbf{E}_t\big(f(\xx_{t+1})\big) &\geq \frac{p_0}{4} h_t\\
\mathbf{E}_t\big(h(\xx_{t+1})\big) &\leq (1-\frac{p_0}{4})h_t
\end{align}


\textbf{Cases $\gamma_{\text{max}}<1$.}  It corresponds necessarily to the choice of an away step. It can be either a drop step, e.g. the considered component along the away vertex will be set to zero and $\gamma_{\text{max}}=\gamma_t^*$ or just a step with $\gamma_{\text{max}}>\gamma_t^*$. As \cite{lacoste2015global} we will consider that for the drop steps it is hard to control the error. Though their number is at worst $\frac{t}{2}$. For non-drop step, the optimal $\gamma_t^*$ is such that:
\begin{eqnarray}
\gamma_t^*\in\underset{\gamma\in[0,\gamma_{\text{max}}]}{\argmin} f(\xx_{t}+\gamma \dd_t)=F(\gamma).
\end{eqnarray}
Though since $\gamma_t^*<\gamma_{\text{max}}$ and $F$ is convex we have:
\begin{eqnarray}
\gamma^*\in\underset{\gamma\in[0,1]}{\argmin} f(\xx_{t}+\gamma \dd_t).
\end{eqnarray}
and we can make the same calculation as in the case $\gamma_{\text{max}}\geq 1$.

\noindent\textbf{cases distinction conclusion:} Denote by $z_t=1$ when we do a drop step at iteration $t$ and 0 otherwise. In fact we have proven that the expectation with respect to the $t^{ith}$ sub-sampling (denote it $S_t$):{\color{red}{reecrire}}
\begin{eqnarray}
\mathbb{E}(h(\xx_{t+1})|x_t,S_t)\leq (1-\rho)^{z_t}h(\xx_t),
\end{eqnarray}
where $\rho=p_0\min(\frac{1}{4},\frac{\mu_f^A}{4 C_f^A})$. Indeed knowing $x_t$ and $S_t$, $z_t$ is not a random variable. Because there are at worth $\frac{t}{2}$ drop steps, $\sum_{i=1}^t{z_t}\geq \frac{1}{2}$. It follows:
\begin{eqnarray}
\mathbb{E}(h(\xx_{t+1}))\leq \mathbb{E}\big((1-\rho)^{\sum_{k=1}^t{z_k}}\big) h(\xx_0)\\
\mathbb{E}(h(\xx_{t+1}))\leq (1-\rho)^{\frac{t}{2}} h(\xx_0)
\end{eqnarray}



%CONVERGENCE RATE
\textit{convergence rate}: After $t$ iteration we have:
\begin{eqnarray}
\mathbb{E}\big( h(\xx^{(t+1)})\big)\leq (1- \frac{p_0^2  \mu_f^A}{4 C_f^A})^{\frac{t}{2}} h(\xx^{(0)})
\end{eqnarray}
\end{proof}



%%%%%%%%%%%%%%%%%%%%%%%%%%%%%%%%%%%%%%%%%%%%%%%%%%%%%%%%%%%%%%%%%%%%%%%%%%%%%%%%%%%%%%%%%%%%%%%%%%%%%%%%%%%%%%%%%%%%%%%%%%%%%%%%%%%%%%%%%%%%%%%%%%%%%%%%%%%
%%%%%%%%%%%%%%%%%%%%%%%%POSSIBILITY TO REFINE THE RATE%%%%%%%%%%%%%%%%%%%%%%%%%%%%%%%%%%%%%%%%%%%%%%%%%%%%%%%%%%%%%%%%%%%%%%%%%%%%%%%%%%%%%%%%%%%%%%%%%%%%
%%%%%%%%%%%%%%%%%%%%%%%%%%%%%%%%%%%%%%%%%%%%%%%%%%%%%%%%%%%%%%%%%%%%%%%%%%%%%%%%%%%%%%%%%%%%%%%%%%%%%%%%%%%%%%%%%%%%%%%%%%%%%%%%%%%%%%%%%%%%%%%%%%%%%%%%%%%

\eqref{eq:lower_bound_expectation} is a bit conservative, theorem \ref{th:raffinment_linear_convergence_rate} provides a finer grained analysis that allows in \ref{ss:numerical_gain} to provide better understanding of the gain of the algorithm.

\begin{theorem}\label{th:raffinment_linear_convergence_rate}

\end{theorem}
\begin{proof}
At iteration $t$, the sub-sample Frank-Wolfe linear oracle will compute $|\mathcal{S}_t|+p$ values of the sequence $(<v;\nabla f(\xx_t)>)_{v\in\mathcal{V}}$ so that \eqref{eq:lower_bound_expectation} transforms into:
\begin{eqnarray}\label{eq:raffined_lower_bound_expectation}
h_t - \textbf{E}_t \big(h_{t+1}\big) \geq \frac{|\mathcal{S}_t|+p}{|\mathcal{V}|} \frac{\tilde{g}_t^2}{8 C_f^A}.
\end{eqnarray}

\end{proof}


%%%%%%%%%%%%%%%%%%%%%%%%%%%%%%%%%%%%%%%%%%%%%%%%%%%%%%%%%%%%%%%%%%%%%%%%%%%%%%%%%%%%%%%%%%%%%%%%%%%%%%%%%%%%%%%%%%%%%%%%%%%%%%%%%%%%%%%%%%%%%%%%%%%%%%%%%%%
%%%%%%%%%%%%%%%%%%%%%%%%WHY PAIR-WISE GAP IS A DUAL GAP%%%%%%%%%%%%%%%%%%%%%%%%%%%%%%%%%%%%%%%%%%%%%%%%%%%%%%%%%%%%%%%%%%%%%%%%%%%%%%%%%%%%%%%%%%%%%%%%%%%%
%%%%%%%%%%%%%%%%%%%%%%%%%%%%%%%%%%%%%%%%%%%%%%%%%%%%%%%%%%%%%%%%%%%%%%%%%%%%%%%%%%%%%%%%%%%%%%%%%%%%%%%%%%%%%%%%%%%%%%%%%%%%%%%%%%%%%%%%%%%%%%%%%%%%%%%%%%%


\footnote{It is an upper bound on the dual gap. Indeed:
\begin{eqnarray}
v_t\in\underset{v\in\mathcal{S}_t}{\argmin } {\langle r_t;v\rangle},
\end{eqnarray} 
so that:
\begin{eqnarray}
g_t^{PW}=\langle s_t;r_t\rangle-\underset{v\in\text{Conv}(\mathcal{S}_t)}{\min } {\langle r_t;v\rangle}.
\end{eqnarray}
Finally since $\xx_t\in\text{Conv}(\mathcal{S}_t)$, we have that:
\begin{eqnarray}
g_t^{PW}\geq \langle s_t-\xx_t;r_t\rangle.
\end{eqnarray}
The right side argument being the FW dual gap, the Pair-Wise dual gap, is an upper bound on the dual gap.
}





\footnote{In this setting the term stochastic refers to variants that uses a stochastic version of the gradient, we follow \cite{Frandi2016} by calling randomized a FW that compute the Linear oracle on a random subset of its vertex.}






% One important point is to distinguish between $\gamma_{\text{max}}$ and $\widetilde\gamma_{\text{max}}$ for the greatest admissible step size along direction $\widetilde\dd_t$ for Classical Away Step or $\dd_t$ for Randomized Away Step:
% \begin{eqnarray}\label{eq:gamma_max_randomized}
% \gamma_{\text{max}} = \left\{
%     \begin{array}{ll}
%         1 & \text{if} \langle - \nabla f(\xx_t);\dd_t^{\text{FW}}\rangle \geq \langle - \nabla f(\xx_t);\dd_t^A\rangle  \\
%         \frac{\alpha_{v_t}}{1-\alpha_{v_t}} & \text{if} \langle - \nabla f(\xx_t);\dd_t^{\text{FW}}\rangle < \langle - \nabla f(\xx_t);\dd_t^A\rangle 
%     \end{array}
% \right.
% \end{eqnarray}
% while:
% \begin{eqnarray}\label{eq:gamma_max_classical}
% \widetilde{\gamma}_{\text{max}} = \left\{
%     \begin{array}{ll}
%         1 & \text{if} \langle-\nabla f(\xx_t);\widetilde\dd_t^{\text{FW}}\rangle \geq \langle-\nabla f(\xx_t);\dd_t^A\rangle  \\
%         \frac{\alpha_{v_t}}{1-\alpha_{v_t}} & \text{if} \langle-\nabla f(\xx_t);\widetilde\dd_t^{\text{FW}}\rangle < \langle-\nabla f(\xx_t);\dd_t^A\rangle 
%     \end{array}
% \right.
% \end{eqnarray}
% where we note that given $\xx_t$ the away direction $\dd^A$ is the same in both version.
%Since we always have $\langle-\nabla f(\xx_t);\dd_t^{FW}\rangle \geq \langle-\nabla f(\xx_t);\widetilde\dd_t^{FW}\rangle$, the Randomized Away FW have a tendency to favor more Away-steps more than its deterministic counter-part.



%%%%%%%%%%%%%%%%%%%%%%%%%%%%%%%%%%%%%%%%%%%%%%%%%%%%%%%%%%%%%%%%%%%%%%%%%%%%%%%%%
%%%%%%%%%%%%%%%%%%%%%%%%%%%%%%%%%%%%%%%%%%%%%%%%%%%%%%%%%%%%%%%%%%%%%%%%%%%%%%%%%
%%%%%%%%%%%%%%%%%%THROWING AWAY NUMERICAL EXPERIMENTS%%%%%%%%%%%%%%%%%%%%%%%%%%%%
%%%%%%%%%%%%%%%%%%%%%%%%%%%%%%%%%%%%%%%%%%%%%%%%%%%%%%%%%%%%%%%%%%%%%%%%%%%%%%%%%
%%%%%%%%%%%%%%%%%%%%%%%%%%%%%%%%%%%%%%%%%%%%%%%%%%%%%%%%%%%%%%%%%%%%%%%%%%%%%%%%%
%%%%%%%%%%%%%%%%%%%%%%%%%%%%%%%%%%%%%%%%%%%%%%%%%%%%%%%%%%%%%%%%%%%%%%%%%%%%%%%%%

%done with interaction matrix where W 
In the following experiments data is simulated from model equation (\ref{eq:model_interaction_FM}) and (\ref{eq:model_interaction_FW}) with no-linear terms. In the first two examples we consider 

We have thus experiments in which we compare both the recovery and the predicting power of the two models with three assumptions on the interaction matrix: sparse, low-rank non positive semi definite and low-rank positive semi-definite. Sparse is the assumption made with Lasso, while low-rank positive semi definite is the assumption for Factorization Machines.\\


%with sparse ground truth
\begin{figure}[!h]
\begin{minipage}{0.32\linewidth}
\includegraphics[width=\linewidth]{images/sp_ground_truth_d10_n100.png}
\end{minipage}
\begin{minipage}{0.32\linewidth}
\includegraphics[width=\linewidth]{images/sp_interactionFM_d10_n100.png}
\end{minipage}
\begin{minipage}{0.32\linewidth}
\includegraphics[width=\linewidth]{images/sp_interactionFW_d10_n100.png}
\end{minipage}
\caption{On the left, the ground truth is a sparse symmetric matrix with null diagonal coefficients. Its coefficients are either $0$ or $1$. It is simulated with $n=100$ data and $d=10$ co-variate. The middle graph shows the recovered interaction matrix with Factorization machines after convergence while the most right one shows the recovered interaction matrix with Randomized Frank-Wolfe after convergence. In this setting }\label{fig:sp_interaction_matrix}
\end{figure}

%plot of prediction, MSE, support recovery with sparse ground truth
\begin{figure}[!h]
\begin{minipage}{0.99\linewidth}
\includegraphics[width=\linewidth]{images/sp_MSE_comparison.png}
\end{minipage}
\caption{ }\label{fig:sp_prediction_comparison}
\end{figure}

\begin{figure}[!h]
\begin{minipage}{0.99\linewidth}
\includegraphics[width=\linewidth]{images/sp_support_comparison.png}
\end{minipage}
\caption{ }\label{fig:sp_support_comparison}
\end{figure}


%\subsection{low rank ground truth}


%with sparse ground truth
\begin{figure}[!h]
\begin{minipage}{0.32\linewidth}
\includegraphics[width=\linewidth]{images/lr_psd_ground_truth_d10_n100.png}
\end{minipage}
\begin{minipage}{0.32\linewidth}
\includegraphics[width=\linewidth]{images/lr_psd_interactionFM_d10_n100.png}
\end{minipage}
\begin{minipage}{0.32\linewidth}
\includegraphics[width=\linewidth]{images/lr_psd_interactionFW_d10_n100.png}
\end{minipage}
\caption{As in figure \ref{fig:sp_interaction_matrix} but with a simulated low rank positive semi definite matrix to which we retrieved . Say that we do cross validation. Say true rank and the one find with CV }\label{fig:lr_psd_interaction_matrix}
\end{figure}

%plot of prediction, MSE, support recovery with sparse ground truth
\begin{figure}[!h]
\begin{minipage}{0.99\linewidth}
\includegraphics[width=\linewidth]{images/lr_psd_MSE_comparison_d10_n100.png}
\end{minipage}
\caption{ }\label{fig:lr_psd_prediction_comparison}
\end{figure}

\begin{figure}[!h]
\begin{minipage}{0.99\linewidth}
\includegraphics[width=\linewidth]{images/lr_psd_support_comparison_d10_n100.png}
\end{minipage}
\caption{ }\label{fig:lr_psd_support_comparison}
\end{figure}

%\subsection{Full rank ground truth in high dimensiona setting}





































%%%%%%%%%%%%%%%%%%%%%%%%%%%%%%%%%%%%%%%%%%%%%%%%%%%%%%%%%%%%%%%%%%%%%%%%%%%
%%%%%%%%%%%%%%%%%%%PAST INTRODUCTION%%%%%%%%%%%%%%%%%%%%%%%%%%%%%%%%%%%%%%%
%%%%%%%%%%%%%%%%%%%%%%%%%%%%%%%%%%%%%%%%%%%%%%%%%%%%%%%%%%%%%%%%%%%%%%%%%%%

\paragraph{Contributions.}
% Paper contribution
The contribution of this paper are two-fold. First, in the interaction selection problem with high dimensional data, we provide alternative to the very expressive factorization machine setting. Namely we propose new randomized versions of the Frank-Wolfe algorithms. %These can be further tuned to the problem as well as they can be up-graded with screening rules. 
Second we provide a convergence analysis of the RFW and RAFW leading in expectation to the same rate as their deterministic counter-part. Namely when applied to generalized strongly convex objective, RAFW converge linearly in expectation.


\paragraph{Related work.}
Algorithm \ref{algo:Randomized_FW_general} in the special case of the lasso problem was first proposed in \citet{Frandi2016}. Here we extend it to any polytope and provide a correct theoretical convergence guarantee. The randomized version of the away step Frank-Wolfe (algorithm \ref{algo:Randomized_away_general}) though is new to our knowledge. The closest approaching algorithm was proposed in \cite{Goldfarb2016}, where they considered an hybrid of the away-step in the block-coordinate setting along with a stochastic Frank-Wolfe. Though it requires a separability of the polytope domain. These randomized version of FW have a similar flavor as the block coordinate FW recently used in a variety of application \citet{lacoste2012block}, or \citet{osokin2016minding}.



% Motivation & Applications
We assume to be in the setting in which the number of dimension, $d$, it too large to be able to store the $d\times d$ matrix of pairwise interactions.

%The use of polynomial regression goes back to 1815~\citep{stigler1974gergonne}. 




%%%%%%%%%%%%%%%%%%%%%%%%%%%%%%%%%%%%%%%%%%%%%%%%%%%%%%%%%%%%%%%%%%%%%%%%%%%
%%%%%%%%%%%%%%%%%%%NUMERICAL GAIN%%%%%%%%%%%%%%%%%%%%%%%%%%%%%%%%%%%%%%%%%%
%%%%%%%%%%%%%%%%%%%%%%%%%%%%%%%%%%%%%%%%%%%%%%%%%%%%%%%%%%%%%%%%%%%%%%%%%%%







\label{para:numerical_gain}
{\color{red}{en cours mais ne donnera probablement rien de bon...}}
Let's compare Theorem \ref{th:RAFW_expectation_result} and \citep[Theorem 8]{lacoste2015global} in the case of the $\ell_1$ ball. 

Each iteration of the RAFW requires to compute $|\mathcal{A}_t|=|\mathcal{S}_t|+p$ coefficients of the gradient. Though the only known way to control $|\mathcal{S}_t|$ is by the number of iteration of the algorithm, so that the cost does not exceed the computation of $t+p$ coefficients of the gradient. When $t+p$ is greater than $\mathcal{V}$, the RAFW falls back to AFW.


\paragraph{Technical discussion}
First remark that \eqref{eq:RAFW_bound_result} implies
\begin{eqnarray}
\mathbb{E}\big[ h(\xx_{t+1})\big]\leq \exp(-\frac{t}{2}p_0\rho_f)h(\xx_0).
\end{eqnarray}

Consider $N$ the number of gradient coefficient computed in AFW. At each iteration there are exactly $|\mathcal{V}|$ such operations. So that from \citep[Theorem 8]{lacoste2015global} we can guarantee the precision
\begin{eqnarray}
\epsilon^{AFW}=\exp(-\frac{1}{2}\floor{\frac{N}{|\mathcal{V}|}}\rho_f)h(\xx_0)
\end{eqnarray}
RAFW with a batch parameter $p$costs at iteration $t$ at worth $\min(t+p,|\mathcal{V}|)$. With $N\leq \frac{(|\mathcal{V}|+1)|\mathcal{V}|}{2}$, we are sure that with a budget $N$, the maximum number of iteration is such that always $\min(t+p,|\mathcal{V}|)=t+p$. With a N-budget and a p-batch the number of RAFW  iteration is
\begin{eqnarray}
t_0=\argmax\{t\in\mathbb{N}~|~\sum_{i=1}^{t}{i+p}\leq N\}
\end{eqnarray}

From that we have $t_0\geq \sqrt{2N}-p$...

For RAFW to be better, it is sufficient to have 
\begin{eqnarray*}
\exp(-\frac{t_0}{2}p_0\rho_f)h(\xx_0)&\leq& \exp(-\frac{1}{2}\floor{\frac{N}{|\mathcal{V}|}}\rho_f)h(\xx_0)\\
t_0 &\geq& \floor{\frac{N}{|\mathcal{V}|}}\frac{|\mathcal{V}|}{p}
\end{eqnarray*}
This last equation will probably not be true because for $t=\frac{N}{p}$, we have $\sum_{i=1}^{t}{i+p}$ much bigger than $N$...


\textbf{This result do not show the benefit of using RAFW because it is very conservative. Indeed it adds to the conservative bound of Theorem \ref{th:RAFW_expectation_result}, another conservative bound on $|\mathcal{S}_t|$, the support of the current iterate.}































\newpage


\section{Various Playground}

{\color{red}{TK:The olde version of lemma B.2}}


%%%%%%%%%%%%%%%%%%%%%%%%%%%%%%%%%%%%%%%%%%%%%%%%%%%%%%%%%%%%%%%%%
%%%%%%%%%%Lemma g_t=tilde g_t%%%%%%%%%%%%%%%%%%%%%%%%%%%%%%%%%%%%
%%%%%%%%%%%%%%%%%%%%%%%%%%%%%%%%%%%%%%%%%%%%%%%%%%%%%%%%%%%%%%%%%
\begin{lemma}\label{lemma:proba_conditional_non_drop_step}
Consider $g_t$ to be the partial pair-wise (PW) dual gap of RAFW at iteration $t$ with sub-sampling parameter $p$ on the constrained polytope $\mathcal{M}=\text{Conv}(\mathcal{V})$, where $\mathcal{V}$ are all extrems points of $\mathcal{M}$. $\tilde{g}_t$ is the PW dual gap of AFW starting at $\xx_t$ on the same polytope. Denote by $z_t$ the binary random variable that equals $0$ when the $t^{th}$ iteration of RAFW makes an away step with $\gamma_{max}<1$, and $1$ otherwise. We have
\begin{eqnarray}
\mathbb{P}(g_t=\tilde{g}_t~|~\xx_t,z_t=1)\geq \frac{p}{|\mathcal{V}|}.
\end{eqnarray}
\end{lemma}


\begin{proof}
Let $g_t^A:=\langle \rr_t;\dd_t^A\rangle$. The event $\{z_t=1\}$ is a partition $A_1 \cup A_2 \cup A_3$ where the $A_i$ are defined by
\begin{eqnarray}
A_1&=&\{g_t\geq g_t^A\}\quad \text{ (performs a FW step)}\\
A_2&=&\{g_t < g_t^A~,~\gamma_{\text{max}}\geq 1\} \quad \text{ (performs away step with $\gamma_{\text{max}} \geq 1$)}\\
A_3&=&\{g_t < g_t^A~,~\gamma_{\text{max}}<1~,~\gamma_t^*<\gamma_{\text{max}}\},
\end{eqnarray}
{\blue FP: it is not clear to me why or what does $A_3$ represent.}
Note that conditionally on $\xx_t$ and on $\{\gamma_{\text{max}}\neq 1\}$, there is no randomness in $\gamma_{\text{max}}$.

We are seeking an upper-bound for P:
\begin{eqnarray*}
P&=&\mathbb{P}(g_t=\tilde{g}_t~|~\xx_t,\{z_t=1\})\\
&=&\frac{\mathbb{P}(g_t=\tilde{g}_t,\{z_t=1\}~|~\xx_t)}{\mathbb{P}(\{z_t=1\}~|~\xx_t)}\\
&=&\frac{\sum_{i=1}^{3}\mathbb{P}(g_t=\tilde{g}_t,A_i~|~\xx_t)}{\sum_{i=1}^{3}\mathbb{P}_t(A_i~|~\xx_t)}\\
P&=&\frac{\sum_{i=1}^3{\mathbb{P}(g_t=\tilde{g}_t~|~x_t,A_i)\mathbb{P}(A_i~|~x_t)}}{\sum_{i=1}^3{\mathbb{P}(A_i~|~x_t)}}.\label{eq:proba_bayes_decomposition}
\end{eqnarray*}

Lets lower-bound the $\mathbb{P}(g_t=\tilde{g}_t~|~x_t,A_i)$. Note that conditionally on $\xx_t$, $\tilde{g}_t$ and $g_t^{\mathcal{A}}$ are deterministic.

For $i=1$, since $\tilde{g}_t \geq g_t$ the event $\{g_t\geq g_t^A\}$ may happen if and only if $\tilde{g}_t \geq g_t^A$. It means that
\begin{eqnarray*}
\mathbb{P}(g_t=\tilde{g}_t~|~x_t,A_1)=1_{\{\tilde{g}_t\geq g_t^A\}} \mathbb{P}(g_t=\tilde{g}_t~|~x_t,A_1)
\end{eqnarray*}
Otherwise the worst case scenario says $g_t=\tilde{g}_t$ with probability $\frac{p}{|\mathcal{V}|}$. We thus have:
\begin{eqnarray}
\mathbb{P}(g_t=\tilde{g}_t~|~x_t,A_1)\geq  1_{\{\tilde{g}_t\geq g_t^A\}} \frac{p}{|\mathcal{V}|}\label{eq:proba_start}.
\end{eqnarray}
Similarly we get:
\begin{eqnarray}
\mathbb{P}(g_t=\tilde{g}_t~|~x_t,A_2)\geq 1_{\{\tilde{g}_t< g_t^A,\gamma_{\text{max}}\geq 1\}} \frac{p}{|\mathcal{V}|}\\
\mathbb{P}(g_t=\tilde{g}_t~|~x_t,A_3)\geq 1_{\{\tilde{g}_t< g_t^A,\gamma_{\text{max}}<1,\gamma_t^*<\gamma_{\text{max}}\}} \frac{p}{|\mathcal{V}|}
\end{eqnarray}

We also have:
\begin{eqnarray}
\mathbb{P}(A_1~|~x_t)=&1_{\{\tilde{g}_t\geq g_t^A\}} \mathbb{P}(A_1~|~x_t)\\
\mathbb{P}(A_2~|~x_t)=&1_{\{\tilde{g}_t< g_t^A,\gamma_{\text{max}}\geq 1\}} \mathbb{P}(A_2~|~x_t)\\
\mathbb{P}(A_3~|~x_t)=&1_{\{\tilde{g}_t< g_t^A,\gamma_{\text{max}}<1,\gamma_t^*<\gamma_{\text{max}}\}} \mathbb{P}(A_3~|~x_t)\label{eq:proba_last}.
\end{eqnarray}
The subtlety here is that when $\tilde{g}_t< g_t^A$ is satisfied, $\gamma_{\text{max}}$ is not random conditionally on $\xx_t$. Indeed it implies $g_t< g_t^A$ and thus an away-step choice.

The combination of \eqref{eq:proba_start}-\eqref{eq:proba_last}  to lower bound \eqref{eq:proba_bayes_decomposition} leaves us with the desired lower-bound:
\begin{eqnarray}
\mathbb{P}_t(g_t=\tilde{g}_t~|~\xx_t,\{z_t=1\})\geq \frac{p}{|\mathcal{V}|}
\end{eqnarray}


\end{proof}









%%%%%%%%%%%%%%%%%%%%%%%%%%%%%%%%%%%%%%%%%%%%%%%%%%%%%%%%%%%%
%%%%%PAST WITH FACTO MACHINES%%%%%%%%%%%%%%%%%%%%%%%%%%%%%
%%%%%%%%%%%%%%%%%%%%%%%%%%%%%%%%%%%%%%%%%%%%%%%%%%%%%%%%%%%%%%




\section{FM and beyond}
{\color{red}{I propose to rewrite the title as "models for learning with interaction". Because it is natural from the beginning that we will not be using factorization machines for inference purposes, e.g. for interaction selection issues? At least if FM literature, there are really about using it for recommender systems which objectives seems mostly to predict! So that finally learning with interaction encapsulates both our interaction selection problem with predicting with the interaction?}}
\paragraph{Factorization Machine:}
To overcome this high memory requirement, factorization machines~\cite{rendle2010factorization} is an increasingly popular approach. It has been successfully applied to recommender systems~\cite{blondel2016polynomial} because it implicitly requires a low rank constrain on the interaction matrix. The model equation for $n$ data $(y_i,\xx_i)\in\mathbb{R}\times\mathbb{R}^d$ is:

\begin{align}\label{eq:model_interaction_FM}
y_i= b+ \langle \ww, \xx_i\rangle + \xx_i^T\boldsymbol{\tilde{W}}\xx_i  \quad,
\end{align}
where $\boldsymbol{W}=PP^T$ with $P\in\mathbb{R}^{d\times k}$ and $\boldsymbol{\tilde{W}}=\boldsymbol{W}-\diag{\boldsymbol{W}}$.

The structure on the interaction matrix makes it unclear\footnote{The explanation of \cite{rendle2010factorization} in paragraph III.A.2) seems to limit the expressiveness of the model to positive definite matrix.} whether or not this model could recover any symmetric interaction matrices $\boldsymbol{W}-\diag{\boldsymbol{W}}$ (\eqref{eq:model_interaction_FM} does not account for squared features). Theorem \ref{th:FM_expressivness} says that indeed model (\ref{eq:model_interaction_FM}) can recover any symmetric interaction matrix. Indeed the set of interaction that it express is all the matrix $f(PP^T)$ for all $P\in\mathbb{R}^{d\times k}$, which by Choleski decomposition equals the set $f(\mathcal{S}_d^+)$.


{\blue FP: this is too much details of FM for an introduction. Ideally, the introduction should explain why the problem we are trying to solve is important, why it hasn't been done before (without going too much into the details) and give an outline of the main contributions. Look at your favorite NIPS/ICML paper to get inspiration :-)}
\begin{theorem}\label{th:FM_expressivness}
Consider the application $f$ on the space of real symmetric matrix $\mathcal{S}_d(\mathbb{R})$:
$$\begin{array}{ccccc}
f & : & \mathcal{S}_d(\mathbb{R}) & \to & \mathcal{S}_d(\mathbb{R}) \\
 & & W & \to & W-\text{diag}(W),
 \\
\end{array}$$
then, by denoting $\mathcal{S}^+_d(\mathbb{R})$ the set of positive semi-definite matrix, we have:
\begin{eqnarray}
f(\mathcal{S}^+)&=&f(\mathcal{S}).
\end{eqnarray}
\end{theorem}

\begin{proof}
Consider any $\boldsymbol{W}_0\in\mathcal{S}_d(\mathbb{R})$. We want to find $\boldsymbol{W}_s\in\mathcal{S}_d^+$ such that $f(\boldsymbol{W}_s)=f(\boldsymbol{W}_0)$.

Immediately we have for $\lambda\in\mathbb{R}$:
\begin{eqnarray}
f(\boldsymbol{W}+\lambda I_d)=f(\boldsymbol{W})
\end{eqnarray}
For $\lambda > \underset{\lambda\in E(\boldsymbol{W})}{\min} |\lambda|$, where $E(\boldsymbol{W})$ denotes the eigenspace of $\boldsymbol{W}$, $\boldsymbol{W}_{\lambda}=\boldsymbol{W}+\lambda I_d$ will be positive semi-definite which concludes the proof.
\end{proof}

%Why not FM
Although FM is tailored for prediction 
has proved to be a computational and predictional success story, it does not adapt efficiently to other settings such as \eqref{eq:model_interaction_FW} when two distinct features vectors are involved. {\color{blue}{Good to give two reasons for doing something else than FM.
\begin{itemize}
\item One is qualitative (cumbersome to compare results on real data?): strange to build interaction selection after FM model, should directly try to do interaction selection
\item Second is that Factorization is not flexible to problem because we may want to forbid some vertex.
\end{itemize}
 }}


More problematically, the model in FM is not tailored to interaction selection problem as the estimated interaction matrix will not naturally set its coefficients to zero. We believe it is crucial to develop efficient training algorithms to solve other model equations, with $\ell_1$ constraints, more flexible and suited to the interaction selection problem. Although it is a simple Lasso problem, the sequel Randomized Frank-Wolfe approach reduces both the memory and computational overhead of training (\ref{eq:model_interaction_FW}) in the high-dimensional setting.

%model equation
\paragraph{Problem statement}
The general model equation for interaction selection  with data $(y_i,\cc_i,\dd_i)\in\mathbb{R}\times\mathbb{R}^c\times\mathbb{R}^d$ would be:
\begin{align}\label{eq:model_interaction_FW}
y_i= \cc_i^T \boldsymbol{W} \dd_i \quad,
\end{align}
with $\boldsymbol{W}\in\mathbb{R}^{c\times d}$ sparse, $\cc_i\in\mathbb{R}^c$ and $\dd_i\in\mathbb{R}^d$. This hypothesis is also tailored to inference issues and situation where the number $n$ of data is insufficient in regard to the number of coefficient of the interaction matrix $\boldsymbol{W}$.

%It encompass the expressiveness of FM model equation
Model equation (\ref{eq:model_interaction_FW}) encompasses many scenario. Adding a column of $1$ in the design matrix of the $\cc_i$ or the $\dd_i$, accounts for linear interaction while $\cc_i=\dd_i$ recovers (\ref{eq:model_interaction_FM}) with another constraint on $\boldsymbol{W}$. When a particular structure on the feature vector, it allows to target specific interaction. For instance in chemotherapy, machine learning is used to predict which association of gene (describes by $c_i$) with a drug\footnote{nothing else than a chemical compound.} (describes by $d_i$) will inhibit the growth of the line-cell describes by $c_i$, when grown with the drug $d_i$. {\blue TK: I will reformulate and give some reference.}

%training the model 
Training such a model with a quadratic loss, imposing an $\ell_1$ constraint to enforce sparsity, is vastly known as lasso and can be equivalently cast as a constrained minimization problem:
\begin{equation}\label{eq:opt}\tag{OPT}
  \argmin_{ \|\boldsymbol{W}\|_1 \leq \beta} \sum_{i=1}^n (y_i - \cc_i^T \boldsymbol{W} \dd_i)^2\quad.
\end{equation}

%Why randomized Frank-Wolfe
\paragraph{Randomized Frank-Wolfe algorithms}
Many algorithms exist to solve \eqref{eq:opt}. Among these, the Frank-Wolfe or conditional gradient method~\citep{frank1956algorithm, jaggi_revisiting_2013} is particularly attractive due to its low memory requirements. For convex polytopes such as the $\ell_1$ ball, the next iteration in this algorithm is a convex combination of the current point with a vertex of the domain. This allows to maintain a \emph{sparse} representation of the coefficients at every iteration.

Here we propose two variants of FW, namely Randomized FW and Randomized Away FW, that answer the following problem:
\begin{eqnarray}\label{eq:general_opt}
  \argmin_{ \xx\in\mathcal{M}} f(x),\quad
\end{eqnarray}
with $f$ a L-smooth function. For the Randomized Away FW, $f$ will be required to be generally strongly convex, e.g. $f(x)=g(Ax)$ with $g$ $\mu$-strongly convex.


The Randomized Frank-Wolfe algorithm is a variation of FW on the $\ell_1$ domain, that reduces the computational requirement of the linear oracle in FW. Although it require other assumptions on the domain, it shares a similar flavor as the Block-coordinate FW in \cite{lacoste2012block} or \cite{osokin2016minding} which works with separable domains. 

Thanks to this computational improvement per iteration, the RFW has an overall low memory requirement and computational cost per iteration that makes it attractive to practitioner across other fields.





































%%%%%%%%%%%%%%%%%%%%%%%%%%%%%%%%%%%%%%%%%%%%%%%%%%%%%%%%%%%%%%%%PREVIOUS LAST PART%%%%%%%%%%%%%%%%%%%%%%%%%%%%%%%%%%%%%%%%%%%%%%%%%%%%%%%%
%%%%%%%%%%%%%%%





{\color{red}{TK: Doing t-iterations of RAFW, there is at least $t/2$ iterations where we can guarantee a strictly positive probability ($\big(\frac{p}{|\mathcal{V}|}\big)^2$) to ensure a geometrical decrease with factor $(1-\rho_f)$ of $h_t$.}}
{\color{red}{Ok let's denote by $A_p^{t}$ the random subset on which to compute the Frank-Wolfe step. We denote by $\mathcal{F}_t=\sigma(x_0,A_p^{1}\cdots A_p^{t-1})$ CHANGE IN THE DEFINITION OF FW. When analyzing RAFW until iteration $t$, we denote by $\mathbb{E}$, the expectation with respect to all the random information until $t$... }}


Denote by $T_i$ the random time at which happens the $i^{th}$ non bad drop step. For ease denote by $\mathcal{T}_{k}=\{T_1,\cdots, T_{k}\}$. We know that $T_{\floor{\frac{t-1}{2}}}$ is smaller than $t$. For $n_0=\floor{\frac{t-1}{2}}$, we can thus write
\begin{eqnarray}
E(h_{t+1})=E(E(h_{t+1}|\mathcal{T}_{n_0})),
\end{eqnarray}
{\blue FP: it is not clear above with respect to what are the expectations computed. Is $E = \mathbb{E}$ or $E = \mathbf{E}$?}{\red TK: ok je vais remplacer tous les E par $\mathbb{E}$}
where $\mathbb{E}$ is the expectation over all the randomness until iteration $t$. {\red TK: I think I inverted the expectation in the "tower property"...}
from which we write $E_{T}=E(h_{t+1}|\mathcal{T}_{n_0})$ and with \eqref{eq:dual_improvement_without_expectation}
\begin{eqnarray*}
E_T&\leq& h_0 E(\prod_{k=0}^{t}{(1-\rho_f\big(\frac{g_t}{\tilde{g}_t}\big)^2 )^{z_t}}~|~\mathcal{T}_{n_0})\\
&\leq& h_0 E(\prod_{k=1}^{n_0}{(1-\rho_f\big(\frac{g_{T_k}}{\tilde{g}_{T_k}}\big)^2 )}~|~\mathcal{T}_{n_0})=H_{n_0},
\end{eqnarray*}
because $z_{T_i}=1$ and otherwise we upper bound the term in the product by $1$.


$\mathcal{R}_t$ being the random information in the $t$-th sub-sampling solely, $\mathcal{F}_t=\sigma(x_0,\mathcal{R}_1\cdots \mathcal{R}_{t-1})$ represents all the information about the RAFW starting at $x_0$ until iteration $t$, but not that of the $t^{ith}$ sub-sampling.

 Since $\mathcal{T}_{n_0}\subset C_{n_0}=\mathcal{F}_{T_{n_0}}\cup\mathcal{T}_{n_0}$, it follows from the tower property
\begin{eqnarray}
H_{n_0}=E(E(\prod_{k=1}^{n_0}{(1-\rho_f\big(\frac{g_{T_k}}{\tilde{g}_{T_k}}\big)^2 )}|~C_{n_0})|~\mathcal{T}_{n_0})
\end{eqnarray}
$\prod_{k=0}^{n_0-1}{(1-\rho_f\big(\frac{g_{T_k}}{\tilde{g}_{T_k}}\big)^2 )}$ is $C_{n_0}$-measurable so that
\begin{eqnarray}
H_{n_0}=E(\prod_{k=1}^{n_0-1}{(1-\rho_f\big(\frac{g_{T_k}}{\tilde{g}_{T_k}}\big)^2 )}           E(1-\rho_f\big(\frac{g_{T_{n_0}}}{\tilde{g}_{T_{n_0}}}\big)^2|C_{n_0})|\mathcal{T}_{n_0}).
\end{eqnarray}
By definition
\begin{eqnarray*}
E(1-\rho_f\big(\frac{g_{T_{n_0}}}{\tilde{g}_{T_{n_0}}}\big)^2|C_{n_0})\leq 1-\rho_f\mathbb{P}(g_{T_{n_0}}=\tilde{g}_{T_{n_0}}~|~C_{n_0}).
\end{eqnarray*}
The event $\{g_{T_{n_0}}=\tilde{g}_{T_{n_0}}\}$ writes
$\{\underset{s\in\mathcal{A}_p}{\text{max }}\langle r_{T_{n_0}};s\rangle=\underset{s\in\mathcal{V}}{\text{max }}\langle r_{T_{n_0}};s\rangle\}$, we thus have

\begin{eqnarray*}
\mathbb{P}(g_{T_{n_0}}=\tilde{g}_{T_{n_0}}~|~C_{n_0}) =\mathbb{P}(g_{T_{n_0}}=\tilde{g}_{T_{n_0}}~|~x_{T_{n_0}},z_{T_{n_0}}=1, T_{n_0} ) .
\end{eqnarray*}
And from Lemma \ref{lemma:proba_conditional_non_drop_step}, we finally get:
\begin{eqnarray}
E((1-\rho_f\big(\frac{g_{T_{n_0}}}{\tilde{g}_{T_{n_0}}}\big)^2|C_{n_0})\leq 1-\rho_f\big(\frac{p}{|\mathcal{V}|}\big)^2 .
\end{eqnarray}

We repeat the process ({\color{red}{TK:maybe I should detail, it is not clear yet }})
\begin{eqnarray}
H_{n_0}\leq (1-\rho_f\big(\frac{p}{|\mathcal{V}|}\big)^2)^{n_0}\\
E(h_{t+1})\leq (1-\rho_f\big(\frac{p}{|\mathcal{V}|}\big)^2)^{\floor{\frac{t-1}{2}}}.
\end{eqnarray}







%%%%%%%%%%%%%%%%%%%%%%%%%%%%%%%%%%%%%%%%%%%%%%%%%%%%%%%%%%%%%%%%%%%%%%%%%%%%%%%%%%%%%%%%%%%%%%%%%%%%%%%
%%%%%%%%%%%%%%%%%%%%%%%%%%%%%%%%%%FORMER MAIN PROOF%%%%%%%%%%%%%%%%%%%%%%%%%%%%%%%%%%%%%%%%%%%%%%%%%%%%
%%%%%%%%%%%%%%%%%%%%%%%%%%%%%%%%%%%%%%%%%%%%%%%%%%%%%%%%%%%%%%%%%%%%%%%%%%%%%%%%%%%%%%%%%%%%%%%%%%%%%%%

%RECOLTER LES FRUITS
At iteration $t$ of RAFW, from \eqref{eq:fruit_second_part} we get
\begin{eqnarray}
\mathbb{E}(h_{t+1}~|~\xx_t,\{z_t=1\})&\leq& (1-\rho_f\mathcal{P}(g_t=\widetilde{g}_t~|~\xx_t,\{z_t=1\})) h_t,
\end{eqnarray}
% AA :square missing here? Cases with g_t \neq \widetilde{g}_t not problematic? Mention explicitly that you only consider only {0,1}
because conditionally on $\xx_t$, $h_t$ is deterministic and we lower-bounded $\frac{g_t}{\widetilde{g}_t}$ by $0$ when it is not equal to 1. Then because of Lemma \ref{lemma:proba_conditional_non_drop_step}
\begin{eqnarray}\label{eq:fruit_expectation_lemma}
\mathbb{E}(h_{t+1}~|~\xx_t,\{z_t=1\})\leq (1-\rho_f\eta^2) h_t,
\end{eqnarray}
where $\eta=\frac{p}{|\mathcal{A}|}$.


%KILL THE BEAST
Consider running RAFW until iteration $t_0$ and denote by $\mathcal{I}_{t_0}$ the set of indices $i$ for which $z_i=1$.

Happily, the number of bad drop step (e.g. $z_i=0$) is upper-bounded by the number of drop-steps which cannot exceed more than half of the iterations. Indeed, as noted in \cite{lacoste2015global}, when denoting by $A_{t_0}$ the number of steps that added a vertex in the expansion and $D_{t_0}$ the number of drop step, we simultaneously have $A_{t_0}+D_{t_0}\leq t_0$ and $0\leq |S^{t_0}|=|S^0|+A_{t_0}-D_{t_0}$. It follows that $D_{t_0} \leq (t + 1 ) / 2$ because we choose $|S^0|=1$.

So that $|\mathcal{I}_{t_0}|\geq \frac{t_0-1}{2}$. Besides, for $t \leq t_0$
% Define \mathcal{I}_{t_0} here instead
\begin{equation}
  \left\{
      \begin{aligned}
        \mathbb{E}(h_{t+1}~|~\mathcal{I}_{t_0})&\leq& (1-\rho_f\eta^2)\mathbb{E}(h_t~|~\mathcal{I}_{t_0})&~&~\text{if } t\in\mathcal{I}_{t_0}\\
        \mathbb{E}(h_{t+1}~|~\mathcal{I}_{t_0})&\leq& \mathbb{E}(h_{t}~|~\mathcal{I}_{t_0})&~&~\text{otherwise}
      \end{aligned}
    \right.
\end{equation}
Indeed the line search guarantee that $h_t$ always decreases for any $t$ so that
\begin{eqnarray}
\mathbb{E}(h_{t+1}~|~\mathcal{I}_{t_0})&\leq& \mathbb{E}(h_{t}~|~\mathcal{I}_{t_0}).
\end{eqnarray}
When $t\in\mathcal{I}_{t_0}$ its means that $\{z_t=1\}$ occurred. Also with respect to the randomness, given $\xx_t$ and the sub-sampling at iteration $t$, $\xx_{t+1}$ is determined. It implies that $\mathbb{E}(h_{t+1}~|~\xx_t,\mathcal{I}_{t_0})=\mathbb{E}(h_{t+1}|\xx_t,\{z_t=1\})$. Finally using \eqref{eq:fruit_expectation_lemma} leads to the following
%AA: Don't we have causality issues with \mathcal{I}_{t_0}, since it is not F_t measurable ??
\begin{eqnarray*}
\mathbb{E}(h_{t+1}~|~\mathcal{I}_{t_0})&=&\mathbb{E}(\mathbb{E}(h_{t+1}~|~\xx_t,\mathcal{I}_{t_0})~|~\mathcal{I}_{t_0})=\mathbb{E}(\mathbb{E}(h_{t+1}|\xx_t,\{z_t=1\})~|~\mathcal{I}_{t_0})\\
&\leq&(1-\rho_f\eta^2)\mathbb{E}(h_t~|~\mathcal{I}_{t_0}).
\end{eqnarray*}

It follows by recurrence that 
\begin{eqnarray}
\mathbb{E}(h_{t_0+1}~|~\mathcal{I}_{t_0})&\leq& (1-\rho_f\eta^2)^{|\mathcal{I}_{t_0}|}h(\xx_0)\leq (1-\rho_f\eta^2)^{\floor{\frac{t-1}{2}}}h(\xx_0)\\
\mathbb{E}(h_{t_0+1})&=&\mathbb{E}(\mathbb{E}(h_{t_0+1}~|~\mathcal{I}_{t_0}))\leq (1-\rho_f\eta^2)^{\floor{\frac{t-1}{2}}}h(\xx_0).
\end{eqnarray}



















%(1-\rho_f \eta^2)^{\max{0,\left\lfloor\frac{t-(s+1)}{2}\right\rfloor}}\\
%(1-\rho_f \eta^2)^{\max{0,\left\lfloor\frac{t-(s-1)}{2}\right\rfloor}}\\
%&\leq& \mathcal{P}(z_1=1)(1-\rho_f \eta^2)^{1+\max{0,\left\lfloor\frac{t-(s+1)}{2}\right\rfloor}}+\mathcal{P}(z_1=0) (1-\rho_f \eta^2)^{\max{0,\left\lfloor\frac{t-(s-1)}{2}\right\rfloor}}\\
%&\leq& (1-\rho_f \eta^2)^{\min\{1+\max{0,\left\lfloor\frac{t-(s+1)}{2}\right\rfloor},\max{0,\left\lfloor\frac{t-(s-1)}{2}\right\rfloor}\}}












%Now we have to upper bound
%$\mathbb{E}(\big(1-\rho_f\big(\frac{g_t}{\widetilde g_t}\big)^2\big)^{z_t}~|~ \xx_{t-1},z_t)$. This depends on the size of the support of $\xx_{t-1}$. 

%\textbf{When $|\mathcal{S}_{t-1}|=0$,} necessarily iteration $t$ will be a FW step and as such $z_t=1$. It results on 
%\begin{eqnarray*}
%\mathbb{E}(\big(1-\rho_f\big(\frac{g_t}{\widetilde g_t}\big)^2\big)^{z_t}~|~ \xx_{t-1},z_t) &\leq& 1-\rho_f \mathcal{P}(g_t=\widetilde g_t~|~,\xx_{t-1},z_t=1)\\
%&\leq& 1-\rho_f \eta^2.
%\end{eqnarray*}
%Applying the recurrence property on \eqref{eq:tower_property} results in 
%\begin{eqnarray}
%\mathbb{E}(\prod_{k=1}^{t}{\big(1-\rho_f\big(\frac{g_k}{\widetilde g_k}\big)^2\big)^{z_k}}) &=& \mathbb{E}\big[ F(t-1,s) \big].
%\end{eqnarray}



%%%%%%%%%%%%%%%%%%%%%%%%%%%%%%%%%%%%%%%%%%%%%%%%%%%%%%%%%%%%%%%%%%%%%%%%%%%%%%%%%%%%%%%%%%%%%%%%%%%%%%%%%%%%%%%%%%%%%%%%%%%%%LEMMA 4 and 5%%%%%%%%%%%%%%%%%%%%%%%%%%%%%%%%%%%%%%%%%%%%%%%%%%%%%%%%%%%%%%%%%%%%%%%%%%%%%%

{\blue FP: definitions that use use on other lemmas should be declared outside the lemma text}

Lemma \ref{lemma:lower_bounding_proba} is an auxiliary result for Lemma \ref{lemma:proba_conditional_non_drop_step}. It makes the bridge between the combinatorial result of Lemma \ref{lemma:proba_worth_case_scenario} and the probabilities appearing in the analysis of RAFW. 
%B3
%%%%%%%%%%%%%%%%%%%%%%%%%%%%%%%%%%%%%%%%%%%%%%%%%%%%%%%%%%%%%%%%%
%%%%%%%%%%Lemma for the probabilities%%%%%%%%%%%%%%%%%%%%%%%%%%%%
%%%%%%%%%%%%%%%%%%%%%%%%%%%%%%%%%%%%%%%%%%%%%%%%%%%%%%%%%%%%%%%%%
\begin{lemma}\label{lemma:lower_bounding_proba}
Let $g_t$ be as defined in Lemma~\ref{lem:progress_direction_sub_away},  $\widetilde{g}_t \defas \underset{\ss\in\mathcal{A}}{\text{max }}\langle -\nabla f(\xx_t);\ss-\vv_t\rangle$. %, where $\mathcal{A}_t$ is defined in Algorithm \ref{algo:Randomized_away_general} as the union of $\mathcal{S}_t$ (the support of $\xx_t$) and $\mathcal{V}_t$ (a subset of size $p$ of $\mathcal{A}\setminus \mathcal{S}_{t}$).
let $\vv_t$ be the away vertex (defined in Algorithm~\ref{algo:Randomized_away_general}) such that $\vv_t \defas \underset{\vv\in\mathcal{S}_t}{\argmax }\langle -\nabla f(\xx_t);\xx_t-\vv\rangle$, and $g_t^A$, the away gap, defined as $
g_t^A\stackrel{\text{def}}{=}\langle -\nabla f(\xx_t);\xx_t-\vv_t\rangle$.
% \begin{eqnarray}\label{eq:def_v_t}
% \vv_t\in\underset{\vv\in\mathcal{S}_t}{\argmax~}{\langle -\nabla f(\xx_t);\xx_t-\vv\rangle}~.
% \end{eqnarray}
Furthermore, let $A_2$ and $A_3$ be defined as  $A_2\defas\{g_t < g_t^A~,~\alpha_{\vv_t}/(1-\alpha_{\vv_t})\geq 1\}$ and $A_3\defas\{g_t < g_t^A~,~\alpha_{\vv_t}/(1-\alpha_{\vv_t})<1~,~\gamma_t^*<\alpha_{\vv_t}/(1-\alpha_{\vv_t})\}$.
Then the following probabilities are verified
\begin{align}
\forall i=2,3~~&\mathcal{P}(g_t=\widetilde{g}_t~|~\xx_t,\widetilde{g}_t< g_t^A,A_i)\geq \frac{p}{|\mathcal{A}|}\label{eq:proba_3}\\
&\mathcal{P}(g_t=\widetilde{g}_t~|~\xx_t, g_t\geq g_t^{A},\widetilde{g}_t\geq g_t^A)\geq \frac{p}{|\mathcal{A}|}\label{eq:proba_1}\\
&\mathcal{P}(g_t\geq g_t^A~|~\xx_t,\widetilde{g}_t\geq g_t^A)\geq \frac{p}{|\mathcal{A}|}\label{eq:proba_2},
\end{align}
\end{lemma}





\begin{proof}
%GENERAL RESULT
The definition of $\vv_t$ in Algorithm~\ref{algo:Randomized_away_general} implies that, conditioned by $\xx_t$, it does not depend on the choice of random subset at iteration $t$. {\blue FP: writing could be improved. I don't understand what the first phrase has to do with the second. Plus, why is your goal that and what does that have to do with the lemma?} Our goal is to show that $\eqref{eq:proba_3}$--$\eqref{eq:proba_2}$ can be lower bounded by
\begin{eqnarray}\label{eq:probability_with_max_sequence}
P=\mathcal{P}(\underset{\ss\in\mathcal{V}_t}{\text{max }}\langle \rr_t;\ss\rangle=\underset{s\in\mathcal{A}}{\text{max }}\langle \rr_t;\ss\rangle~|~(\langle \rr_t;\ss\rangle)_{s\in\mathcal{A}})~.
\end{eqnarray}
{\blue FP: I don't understand the conditioning on previous eq., why not conditioning on $\xx_t$?}
By definition of $\mathcal{V}_t$ on line \ref{line:def_A_t} in RAFW, we have $|\mathcal{V}_t|=|\mathcal{S}_t|+p$. Since we do not control the support $\mathcal{S}_t$ of $\xx_t$ {\blue (FP: Don't understand what you mean here)}, we loosely lower bound  $\mathcal{V}_t$ by $p$. We apply Lemma \ref{lemma:proba_worth_case_scenario} to the sequence $(\langle \rr_t;\ss\rangle)_{s\in\mathcal{A}}$ to get 
\begin{eqnarray}
P\geq \frac{p}{|\mathcal{A}|},
\end{eqnarray}
which is the desired lower bound.

{\blue FP: make sure all vectors are boldface}


%TRANSFORMATION FOR 1
\noindent\textbf{Case of \eqref{eq:proba_1}}. Lets denote it {\blue (FP: denote what?) } by $P_1$. By definition of $g_t$ and $\widetilde{g}_t$, with $\rr_t=-\nabla f(\xx_t)$, we have:
\begin{align}
&P_1=\mathcal{P}(\underset{\ss\in\mathcal{V}_t}{\text{max }}\langle \rr_t;s-\vv_t\rangle=\underset{s\in\mathcal{A}}{\text{max }}\langle \rr_t;s-\vv_t\rangle~|~\xx_t, \underset{\ss\in\mathcal{V}_t}{\text{max }}\langle \rr_t;s-\vv_t\rangle \geq g_t^A,\underset{s\in\mathcal{A}}{\text{max }}\langle \rr_t;s-\vv_t\rangle\geq g_t^A)\\
&P_1=\mathcal{P}(\underset{\ss\in\mathcal{V}_t}{\text{max }}\langle \rr_t;\ss\rangle=\underset{s\in\mathcal{A}}{\text{max }}\langle \rr_t;\ss\rangle~|~\xx_t, \underset{\ss\in\mathcal{V}_t}{\text{max }}\langle \rr_t;\ss\rangle \geq C_0 ,\underset{s\in\mathcal{A}}{\text{max }}\langle \rr_t;\ss\rangle\geq C_0),
\end{align}
{\blue (FP: when its a chain of equalities or inequalities, one usually does not repeat the left hand side, as is done e.g. on~\eqref{eq:inequ_p_2}. Do same above and in other places where this is the case) }
with $C_0 \defas g_t^A+\langle \rr_t;v_t\rangle$ and $\rr_t$ are totally determined {\blue (FP: not a fan of this phrase (totally determined), as it also depends on $f$ and many other things and sounds vague to me. Would replace with something along the lines of ``does not depend on the random sampling at iteration $t$'' [because I think this is the crucial part, right?] )} by $\xx_t$. Bayes formula leads to
\begin{align}
P_1=\frac{\mathcal{P}(\{\underset{\ss\in\mathcal{V}_t}{\text{max }}\langle \rr_t;\ss\rangle=\underset{s\in\mathcal{A}}{\text{max }}\langle \rr_t;\ss\rangle \}\cap\{ \underset{\ss\in\mathcal{V}_t}{\text{max }}\langle \rr_t;\ss\rangle \geq C_0\} ~|~\xx_t,\underset{s\in\mathcal{A}}{\text{max }}\langle \rr_t;\ss\rangle\geq C_0)}{\mathcal{P}(\underset{\ss\in\mathcal{V}_t}{\text{max }}\langle \rr_t;\ss\rangle \geq C_0 ~|~\xx_t,\underset{s\in\mathcal{A}}{\text{max }}\langle \rr_t;\ss\rangle\geq C_0)}
\end{align}
Conditionally on $\{\underset{s\in\mathcal{A}}{\text{max }}\langle \rr_t;\ss\rangle\geq C_0\}$, we have
$\{\underset{\ss\in\mathcal{V}_t}{\text{max }}\langle \rr_t;\ss\rangle=\underset{s\in\mathcal{A}}{\text{max }}\langle \rr_t;\ss\rangle \}\subset \{\underset{\ss\in\mathcal{V}_t}{\text{max }}\langle \rr_t;\ss\rangle \geq C_0\}$ {\blue (FP: strictly speaking the previous are a set of booleans, I think something like $\{t\, |\, \underset{\ss\in\mathcal{V}_t}{\text{max }}\langle \rr_t;\ss\rangle=\underset{s\in\mathcal{A}}{\text{max }}\langle \rr_t;\ss\rangle \}\subset \{t\, |\, \underset{\ss\in\mathcal{V}_t}{\text{max }}\langle \rr_t;\ss\rangle \geq C_0\}$) would be more correct)} which leads to
\begin{align}
&P_1=\frac{\mathcal{P}(\underset{\ss\in\mathcal{V}_t}{\text{max }}\langle \rr_t;\ss\rangle=\underset{s\in\mathcal{A}}{\text{max }}\langle \rr_t;\ss\rangle ~|~\xx_t,\underset{s\in\mathcal{A}}{\text{max }}\langle \rr_t;\ss\rangle\geq C_0)}{\mathcal{P}(\underset{\ss\in\mathcal{V}_t}{\text{max }}\langle \rr_t;\ss\rangle \geq C_0 ~|~\xx_t,\underset{s\in\mathcal{A}}{\text{max }}\langle \rr_t;\ss\rangle\geq C_0)}\\
&P_1\geq  \mathcal{P}(\underset{\ss\in\mathcal{V}_t}{\text{max }}\langle \rr_t;\ss\rangle=\underset{s\in\mathcal{A}}{\text{max }}\langle \rr_t;\ss\rangle ~|~\xx_t,\underset{s\in\mathcal{A}}{\text{max }}\langle \rr_t;\ss\rangle\geq C_0).
\end{align}

$C_0$ and the sequence $(\langle \rr_t;\ss\rangle)_{s\in\mathcal{A}}$ are determined by $\xx_t$ so that {\blue (I don't get why)}
\begin{eqnarray}
P_1\geq\mathcal{P}(\underset{\ss\in\mathcal{V}_t}{\text{max }}\langle \rr_t;\ss\rangle=\underset{s\in\mathcal{A}}{\text{max }}\langle \rr_t;\ss\rangle~|~(\langle \rr_t;\ss\rangle)_{s\in\mathcal{A}}).
\end{eqnarray}
It is the claimed lower-bound of \eqref{eq:probability_with_max_sequence}.

%TRANSFORMATION FOR 2
\noindent\textbf{Case of \eqref{eq:proba_2}}. Lets denote 
\begin{eqnarray}
P_2&=&\mathcal{P}(g_t\geq g^A_t~|~\xx_t , \widetilde{g}_t \geq g_t^{A}).
\end{eqnarray}
Because, conditionally on $\{\widetilde{g}_t\geq g_t^A\}$, $\{g_t=\widetilde{g}_t\}\subset\{g_t\geq g_t^{A}\}$, we have
\begin{eqnarray}\label{eq:inequ_p_2}
P_2&\geq& \mathcal{P}(g_t=\widetilde{g}_t~|~\xx_t,\widetilde{g}_t\geq g_t^A),\\
&\geq&\mathcal{P}(\underset{\ss\in\mathcal{V}_t}{\text{max }}\langle \rr_t;\ss\rangle=\underset{s\in\mathcal{A}}{\text{max }}\langle \rr_t;\ss\rangle~|~\xx_t, \underset{s\in\mathcal{A}}{\text{max }}\langle \rr_t;\ss\rangle\geq C_0)\\
&\geq&\mathcal{P}(\underset{\ss\in\mathcal{V}_t}{\text{max }}\langle \rr_t;\ss\rangle=\underset{s\in\mathcal{A}}{\text{max }}\langle \rr_t;\ss\rangle~|~(\langle \rr_t;\ss\rangle)_{s\in\mathcal{A}}).
\end{eqnarray}

%TRANSFORMATION FOR 3
\noindent\textbf{Case of \eqref{eq:proba_3}}. In the case of $A_3$, we denote \eqref{eq:proba_3} by $P_3$ (case with $A_2$ is easier). In the same fashion as for $P_1$, we can rewrite it as
\begin{eqnarray*}
P_3&=&\mathcal{P}(\underset{\ss\in\mathcal{V}_t}{\text{max }}\langle \rr_t;\ss\rangle=\underset{s\in\mathcal{A}}{\text{max }}\langle \rr_t;\ss\rangle~|~\xx_t, \underset{\ss\in\mathcal{V}_t}{\text{max }}\langle \rr_t;\ss\rangle < C_0 ,\underset{s\in\mathcal{A}}{\text{max }}\langle \rr_t;\ss\rangle<C_0,\alpha_{\vv_t}/(1-\alpha_{\vv_t})< 1, \gamma_t^*<\alpha_{\vv_t}/(1-\alpha_{\vv_t})).\\
\end{eqnarray*}
Here because the event $\{\underset{\ss\in\mathcal{V}_t}{\text{max }}\langle r_t;s\rangle < C_0\}$ is a consequence of $\{\underset{s\in\mathcal{A}}{\text{max }}\langle \rr_t;\ss\rangle < C_0\}$, we have
\begin{eqnarray*}
P_3&=&\mathcal{P}(\underset{\ss\in\mathcal{V}_t}{\text{max }}\langle \rr_t;\ss\rangle=\underset{s\in\mathcal{A}}{\text{max }}\langle \rr_t;\ss\rangle~|~\xx_t ,\underset{s\in\mathcal{A}}{\text{max }}\langle \rr_t;\ss\rangle < C_0,\alpha_{\vv_t}/(1-\alpha_{\vv_t})< 1, \gamma_t^*<\alpha_{\vv_t}/(1-\alpha_{\vv_t}))\\
%&=&\mathcal{P}(\underset{\ss\in\mathcal{V}_t}{\text{max }}\langle \rr_t;\ss\rangle=\underset{s\in\mathcal{A}}{\text{max }}\langle \rr_t;\ss\rangle~|~\xx_t,\frac{\alpha_{v_t}}{1-\alpha_{v_t}}< 1,\gamma_t^*<\frac{\alpha_{v_t}}{1-\alpha_{v_t}})\\
%&=&\mathcal{P}(\underset{\ss\in\mathcal{V}_t}{\text{max }}\langle \rr_t;\ss\rangle=\underset{s\in\mathcal{A}}{\text{max }}\langle \rr_t;\ss\rangle~|~\xx_t)\\
&=&\mathcal{P}(\underset{\ss\in\mathcal{V}_t}{\text{max }}\langle \rr_t;\ss\rangle=\underset{s\in\mathcal{A}}{\text{max }}\langle \rr_t;\ss\rangle~|~(\langle \rr_t;\ss\rangle)_{s\in\mathcal{A}}).
\end{eqnarray*}
This is true because $C_0$ and $\alpha_{v_t}$ are, by definition, determined by $\xx_t$. Hence all the conditioning in the above probability are just deterministic constrains on the sequence $(\langle \rr_t;\ss\rangle)_{s\in\mathcal{A}})$. It remains to prove that it is the case for $\gamma_t^*$ which is defined by
\begin{eqnarray}
\gamma_t^*\in\underset{\gamma\in[0;\frac{\alpha_{\vv_t}}{1-\alpha_{\vv_t}}]}{\argmin~} f(\xx_t+\gamma \dd_t^A),
\end{eqnarray}
so that it is entirely determined by $\xx_t$, justifying the last equality.
\end{proof}



In the second part of the main proof we ensure a geometric decrease only when $g_t=\widetilde{g}_t$ and $z_t=1$. This last event correspond to not doing a particular type of \textit{drop step} in RAFW that we will name as \textit{bad drop step}. The following lemma helps quantifying the probability of $g_t=\widetilde{g}_t$ to happen when there is a chance to ensure geometrical decrease.



%%%%%%%%%%%%%%%%%%%%%%%%%%%%%%%%%%%%%%%%%%%%%%%%%%%%%%%%%%%%%%%%%
%%%%%%%%%%Lemma g_t=tilde g_t%%%%%%%%%%%%%%%%%%%%%%%%%%%%%%%%%%%%
%%%%%%%%%%%%%%%%%%%%%%%%%%%%%%%%%%%%%%%%%%%%%%%%%%%%%%%%%%%%%%%%%
\begin{lemma}\label{lemma:proba_conditional_non_drop_step}
Consider $g_t$ (defined in Lemma~\ref{lem:progress_direction_sub_away}) to be the partial pair-wise (PW) dual gap of RAFW at iteration $t$ with sub-sampling parameter $p$ on the constrained polytope $\mathcal{M}=\conv(\mathcal{A})$, where $\mathcal{A}$ are all extremes points of $\mathcal{M}$. $\widetilde{g}_t$ (defined in Lemma~\ref{lemma:lower_bounding_proba}) is the pairwise dual gap of AFW starting at $\xx_t$ on the same polytope. Denote by $z_t$ the binary random variable that equals $0$ when the $t^{th}$ iteration of RAFW makes an away step that is a drop step with $\gamma_{max}<1$, and $1$ otherwise (a bad drop step). Then we have the following bound on the probability of not making a bad drop step
\begin{eqnarray}
\mathcal{P}(g_t=\widetilde{g}_t~|~\xx_t,z_t=1)\geq \Big(\frac{p}{|\mathcal{A}|}\Big)^2.
\end{eqnarray}
\end{lemma}


\begin{proof}
%INTRODUCTION OF THE PARTITION ON A_I
Recall that $g_t^A \defas \langle \rr_t;\dd_t^A\rangle$. By definition $\{z_t=0\}=\{g_t<g_t^A,\gamma_{\text{max}}<1,\gamma_t^*=\gamma_{\text{max}}\}$   so that its complementary $\{z_t=1\}$ can be expressed as the partition $A_1 \cup A_2 \cup A_3$ where the $A_i$ are defined by
\begin{eqnarray}
A_1&=&\{g_t\geq g_t^A\}\quad \text{ (performs a FW step)}\\
A_2&=&\{g_t < g_t^A~,~\alpha_{\vv_t}/(1-\alpha_{\vv_t})\geq 1\} \quad \text{ (performs away step with $\gamma_{\text{max}} \geq 1$)}\\
A_3&=&\{g_t < g_t^A~,~\alpha_{\vv_t}/(1-\alpha_{\vv_t})<1~,~\gamma_t^*<\alpha_{\vv_t}/(1-\alpha_{\vv_t})\}.
\end{eqnarray}

First note that in the case of $A_2$ and $A_3$, $\gamma_{\text{max}}=\alpha_{\vv_t}/(1-\alpha_{\vv_t})$. Though the right hand side formulation highlights that it is entirely determined by $\xx_t$.

 From a higher level perspective these cases are those for which we can guarantee a geometrical decrease of $h_t$. By definition, the $A_i$ are disjoints. $A_1$ represents a choice of a FW step in RAFW contrary to $A_2$ and $A_3$ which stands for an away step choice in RAFW. $A_2$ is an away step for which there is enough potential mass ($\gamma_{\text{max}}>1$) to move along the away direction. $A_3$ encompasses the situations where there is not a lot of mass along the away direction ($\gamma_{\text{max}}<1$) but which is not a drop step, e.g. the amount of mass is not a limit for the descent.


%EXPLANATION OF GOAL
Our goal is to lower bound $P=\mathcal{P}(g_t=\widetilde{g}_t~|~\xx_t,z_t=1)$. Since every probability will be conditionally on $\xx_t$, it is important to notice that $g_t^A$,$\widetilde{g}_t$ and $\alpha_{v_t}$ are entirely determined by $\xx_t$. With Bayes formula, and because the $A_i$ are disjoints, we can decompose
\begin{eqnarray}
P&=&\mathcal{P}(g_t=\widetilde{g}_t~|~\xx_t,\{z_t=1\})\nonumber\\
%&=&\frac{\mathcal{P}(\{g_t=\widetilde{g}_t\}\cap\{z_t=1\}~|~\xx_t)}{\mathcal{P}(\{z_t=1\}~|~\xx_t)}\nonumber\\
%&=&\frac{\sum_{i=1}^{3}\mathcal{P}(\{g_t=\widetilde{g}_t\}\cap A_i~|~\xx_t)}{\sum_{i=1}^{3}\mathcal{P}(A_i~|~\xx_t)}\nonumber\\
&=&\frac{\sum_{i=1}^3{\mathcal{P}(g_t=\widetilde{g}_t~|~\xx_t,A_i)\mathcal{P}(A_i~|~\xx_t)}}{\sum_{i=1}^3{\mathcal{P}(A_i~|~\xx_t)}}.\label{eq:proba_bayes_decomposition}
\end{eqnarray}

{\color{red}{TK: I write conditional probabilities on event that may have a probability zero to happen (so that it can hurt some people feelings?) but it does not change anything in the calculation.}}

%WHY A CASE DISTINCTION
By definition of $g_t$ in Lemma \ref{lem:progress_direction_sub_away} and of $\widetilde{g}_t$ in Lemma \ref{lemma:lower_bounding_proba}, $g_t\leq \widetilde{g}_t$, so that when measuring the probability of an event like $\{g_t=\widetilde{g}_t\}$ conditionally on $\{g_t\leq g_t^A\}$ it will naturally depends on whether or not $\widetilde{g}_t\geq g_t^A$ is satisfied. Hence the following case distinction.

{\blue Make sure all vectors are in boldface letter, many $\xx_t$ below are not}

%%%%%%%%%%%%%%%FIRST CASE%%%%%%%%%%%%%%%%%%%%%%%%%%%%%%%%%%%%%%%%%%%%%%%%%
\noindent\textbf{Case $\widetilde{g}_t < g_t^A$.} %Since $g_t\leq \widetilde{g}_t$, it implies that $g_t\leq g_t^A$ and $P$ writes as
\begin{eqnarray}
P=\frac{\sum_{i=1}^3{\mathcal{P}(g_t=\widetilde{g}_t~|~x_t,A_i,\widetilde{g}_t < g_t^A)\mathcal{P}(A_i~|~x_t,\widetilde{g}_t < g_t^A)}}{\sum_{i=1}^3{\mathcal{P}(A_i~|~x_t,\widetilde{g}_t < g_t^A)}}.
\end{eqnarray}
Recall that $A_1=\{g_t\geq g_t^A\}$. Since we always have $g_t\leq \widetilde{g}_t$ by definition of $\widetilde{g}_t$, conditionally on $\{\widetilde{g}_t < g_t^A\}$, $A_1$ cannot happen {\blue (FP: wouldn't it be clearer to say has probability zero?)} and so the above simplifies to 
\begin{eqnarray*}
P=\frac{\sum_{i=2}^3{\mathcal{P}(g_t=\widetilde{g}_t~|~x_t,A_i,\widetilde{g}_t < g_t^A)\mathcal{P}(A_i~|~x_t,\widetilde{g}_t < g_t^A)}}{\sum_{i=2}^3{\mathcal{P}(A_i~|~x_t,\widetilde{g}_t < g_t^A)}}.
\end{eqnarray*}
In addition, from Lemma \ref{lemma:lower_bounding_proba}, using the lower bound on \eqref{eq:proba_3}, for $i=2,3$ we have $\mathcal{P}(g_t=\widetilde{g}_t~|~x_t,A_i,\widetilde{g}_t < g_t^A)\geq \frac{p}{|\mathcal{A}|}$ so that:
\begin{eqnarray*}
P\geq \frac{p}{|\mathcal{A}|}     \frac{\sum_{i=2}^3{\mathcal{P}(A_i~|~x_t,\widetilde{g}_t < g_t^A)}}
{\sum_{i=2}^3{\mathcal{P}(A_i~|~x_t,\widetilde{g}_t \leq g_t^A)}}
=\frac{p}{|\mathcal{A}|}
\end{eqnarray*}

%%%%%%%%%%%%%%%SECOND CASE%%%%%%%%%%%%%%%%%%%%%%%%%%%%%%%%%%%%%%%%%%%%%%%%%%
\noindent\textbf{Case $\widetilde{g}_t \geq g_t^A$.} $P$ rewrites as
\begin{eqnarray}
P=\frac{\sum_{i=1}^3{\mathcal{P}(g_t=\widetilde{g}_t~|~x_t,A_i,\widetilde{g}_t \geq g_t^A)\mathcal{P}(A_i~|~x_t,\widetilde{g}_t \geq g_t^A)}}{\sum_{i=1}^3{\mathcal{P}(A_i~|~x_t,\widetilde{g}_t \geq g_t^A)}}.
\end{eqnarray}
In this case $\mathcal{P}(g_t=\widetilde{g}_t~|~x_t,A_i,\widetilde{g}_t \geq g_t^A)=0$ for $i=2,3$ because $A_i$ implies $g_t\leq g_t^A$. So that when $\widetilde{g}_t \geq g_t^A$ it is then impossible for $g_t$ to equal $\widetilde{g}_t$. 
\begin{eqnarray*}
P=\frac{\mathcal{P}(g_t=\widetilde{g}_t~|~x_t,A_1,\widetilde{g}_t \geq g_t^A)\mathcal{P}(A_1~|~x_t,\widetilde{g}_t \geq g_t^A)}{\sum_{i=1}^3{\mathcal{P}(A_i~|~x_t,\widetilde{g}_t \geq g_t^A)}}.
\end{eqnarray*}
Using the lower on \eqref{eq:proba_1} in lemma \ref{lemma:lower_bounding_proba}, e.g. to lower bound $\mathcal{P}(g_t=\widetilde{g}_t~|~x_t,A_1,\widetilde{g}_t \geq g_t^A)$, we first get
\begin{eqnarray*}
P\geq \frac{p}{|\mathcal{A}|}\frac{\mathcal{P}(A_1~|~x_t,\widetilde{g}_t \geq g_t^A)}{\sum_{i=1}^3{\mathcal{P}(A_i~|~x_t,\widetilde{g}_t \geq g_t^A)}}.
\end{eqnarray*}
Because the $A_i$ are disjoints, $\sum_{i=1}^3{\mathcal{P}(A_i~|~x_t,\widetilde{g}_t \geq g_t^A)}\leq 1$ so that
\begin{eqnarray*}
P\geq\frac{p}{|\mathcal{A}|}\mathcal{P}(A_1~|~x_t,\widetilde{g}_t \geq g_t^A).
\end{eqnarray*}
Finally we use again Lemma \ref{lemma:lower_bounding_proba} for \eqref{eq:proba_2} to lower bound $\mathcal{P}(g_t\geq g_t^A~|~x_t,\widetilde{g}_t \geq g_t^A)$ to get
\begin{eqnarray}\label{eq:lower_bounding_last_case}
P\geq \Big(\frac{p}{|\mathcal{A}|}\Big)^2.
\end{eqnarray}

%%%%%%%%%%%%%%%CONCLUSION%%%%%%%%%%%%%%%%%%%%%%%%%%%%%%%%%%%%%%%%%%%%%%%%%%
\noindent\textbf{Conclusion:} it is hard to respectively count the occurrences of $\{\widetilde{g}_t\geq g_t^A\}$ and $\{\widetilde{g}_t<g_t^A\}$. Consequently we are stuck at lower bounding P in the all cases as in the particular case of \eqref{eq:lower_bounding_last_case}. This will directly impact the rate of convergence.


\end{proof}










































%%%%%%%%%%%%%%%%%%%%%%%%%%%%%%%%%%%%%%%%%%%%%%%%%%%%%%%%%%%%%%%%%%%%%%%%%
%%%%%%%%%%%%%%%%%%%%%PAST NUMERICAL RESULTS%%%%%%%%%%%%%%%%%%%%%%%%%%%%%%
%%%%%%%%%%%%%%%%%%%%%%%%%%%%%%%%%%%%%%%%%%%%%%%%%%%%%%%%%%%%%%%%%%%%%%%%%


\subsection{Interaction selection}
%Interaction selection
Modeling the relationship between an independent variable $\xx$ and a dependent or target variable $\yy$ as a polynomial in $\xx$ is a classical approach in statistics that has been used to describe nonlinear phenomena such as the growth rate of tissues~\citep{shaw2006intellectual}, the distribution of carbon isotopes in lake sediments~\citep{barker200114}, and the progression of disease epidemics~\citep{greenland1995dose}. 
This approach is often referred to as polynomial expansion or polynomial regression. It allows to model a non-linear response function while maintaining the interpretability of a linear model: once the model is estimated, the coefficients correspond to either variables (degree 1 monomial) or products of variables.

%Large scale issues
Unfortunately, this approach cannot be applied to modern large-scale data-sets due to the increasing number of variables, which scales as $\mathcal{O}(d^t)$, where $d$ is the number of features and $t$ is
the order of interactions considered. It is not uncommon for modern data-sets to have beyond one million features. However, storing a dense square matrix with this number of rows and column would exhaust the memory of today's most powerful supercomputer. 

%Interaction selection as a Lasso problem
Interaction selection can be addressed as a Lasso problem {\blue FP: needs explanation}. Many works have been carried out to improve the efficiently of Lasso solvers. Efficient algorithm often rely on coordinate descent and extension \citep{friedman2007pathwise,johnson2017stingycd} which requires to store all the possible interaction along the algorithm even-though the solution ends up sparse. One line of work to reduce the computational cost of optimizing over non-active feature is known as screening rules \citep{ghaoui2010safe}. There are many variation between screening out feature that are guaranteed to be non-active (safe screening rules) and heuristically screening out features that are not necessarily non-active \citep{fercoq2015mind,xiang2017screening}. Without structure on the screened features, these approaches still require to store the potentially active as well as the screened one, it only reduces the computational cost. Some work have been directed toward addressing this memory constrain with tree pattern, but to deal with orders of interaction much greater than 2 \citep{nakagawa2015safe}.


\paragraph{Sub-sample oracle for \eqref{eq:opt}.}
%computationally interesting for the l^1-ball
In the particular case of the $\ell_1$-ball, algorithm \ref{algo:Randomized_FW_general} reduces the computational burden per iteration. Indeed the sub-sampled linear oracle in line \ref{algo:sub_sampled_linear_oracle} transforms into $\boldsymbol{v}_{k}= e_{i^*}$ where $i^*$ satisfies:
\begin{align}
i^* \in \argmin_{i\in I_p} |\nabla f(\xx_{k})|_i,
\end{align}
where $I_p$ is a random subset of size $p$ the index $[1;\cdots;d]$ of the coordinate (with $\xx_{k}\in\mathbb{R}^d$). We observe that we only need to compute the gradient on a batch of its coordinate.

\paragraph{Exact line-search.}
{\red TK: can I skip that completely?}
Two computational details that are essentials for the competitiveness of the algorithm in the case of $\eqref{eq:opt}$. By iteratively keeping track of the residuals, it requires a light computational cost to do the exact line-search and to sub-sample the gradient on a batch.\\

\eqref{eq:opt} can be rewritten in short as:

\begin{equation}\label{eq:opt_vectorize}
  \argmin_{ \|\boldsymbol{W}\|_1 \leq \beta} ||Y-\text{diag}(XWX^T)||_2^2,
\end{equation}
where $X$ is the design matrix.\\

Frank-Wolf updates atom-wise $a^*=\epsilon e_{i^*,j^*}$. The residual\footnote{It is called method of residual in \cite{Frandi2016}} $R_t=Y-\text{diag}(XW_tX^T)$, can then be updated by:
\begin{equation}
R_{t+1}=R_{t}-\epsilon X_{:,i^*} \odot X_{:,j^*}.
\end{equation}
Its cost is $\mathcal{O}(n)$. A coordinated of the gradient is given by:
\begin{equation}
(\nabla f(W_t))_{i,j}=-2-\nabla f(\xx_t)^T(X_{:,i} \odot X_{:,j}).
\end{equation}
Without keeping in memory any previous gradient coefficient requires then a computational effort of $\mathcal{O}(np)$ to calculate the gradient on $p$ vertices. It is dimension-free.\\

The loss being quadratic, the line-search can be done in a close-form which also does not require much computational effort. In the update $W_{t+1}=W_t+\gamma (s_t-W_t)$; with $d_{FW}=(s_t-W_t)$, the best choice of $\gamma\in[0,1]$ is:
\begin{equation}
\gamma^*=\text{proj}_{[0,1]}\frac{R_t^T(\text{diag}(Xd_{FW}X^T))}{||\text{diag}(Xd_{FW}X^T)||_2^2}.
\end{equation}
Here it requires the computation of the n-dimensional vector $\text{diag}(Xd_{FW}X^T)$ which can be evaluated knowing $R_t$ with an additional cost of $\mathcal{O}(n)$. Overall the exact line-search has a $\mathcal{O}(n)$. \textbf{Each iteration cost is then dominated by computing a sub-sample batch of the gradient.}








%\begin{figure}[!h]
%\begin{minipage}{0.49\linewidth}
%\includegraphics[width=\linewidth]{images/R_outside_d30_dual_gap.png}
%\end{minipage}
%\begin{minipage}{0.49\linewidth}
%\includegraphics[width=\linewidth]{images/R_outside_d30_support.png}
%\end{minipage}

%\begin{minipage}{0.49\linewidth}
%\includegraphics[width=\linewidth]{images/RA_outside_d30_dual_gap.png}
%\end{minipage}
%\begin{minipage}{0.49\linewidth}
%\includegraphics[width=\linewidth]{images/RA_outside_d30_support.png}
%\end{minipage}

%\caption{Solving \eqref{eq:opt} with $d=10$ and $n=100$ on synthetic data, where the true interaction matrix is sparse with zero diagonal and sparsity ratio $0.1$.\\
%The left side figures show the convergence evolution of the Frank-Wolfe dual gap (that is not naturally computed in randomized versions) against the cumulative number of computed gradient coefficient along the algorithm. We observe that Randomized version performs much better with that respect that there deterministic counter-part.\\
%The right side figures exhibit the size of the support iterate against the guaranteed precision by the Frank-Wolfe dual gap.
%}\label{fig:RFW_vs_FW}
%\end{figure}




























\begin{figure}[!h]
\begin{minipage}{0.99\linewidth}
\includegraphics[width=\linewidth]{images/FW_RFW_outside_d20_n100_sparsity005.png}
\end{minipage}

\caption{Solving the interaction selection problem with $d=20$ and $n=100$ on synthetic data, where the true interaction matrix is sparse with zero diagonal and sparsity ratio $0.05$.The left panel figures display the evolution of the FW dual gap against the number of gradient coefficients computed. Sub-sampling outperforms clearly the deterministic away steps. {\blue FP: try to optimize the space in this figure. Currently its mostly empty with a bit of information in the corners. Change x and y scales to make the information well centered. Also, would be great to have the curves until $10^{-2}$ or $10^{-3}$}}\label{fig:RFW_vs_FW}
\end{figure}
















%\paragraph{Other randomized variants.} There exists other linearly-convergent variants of FW. A notable expample is the pairwise FW \citep{lacoste2015global}. 
%As we did for RAFW, it is possible to derive a randomized version of this algorithm. The only needed change is
%\begin{algorithm}[h]
%  \dots as in Algorithm \ref{algo:Randomized_away_general}, replacing lines 9 to 13 by:
%  $\dd_t=\ss_t-\vv_t$, and $\gamma_{\text{max}}=\alpha_{\vv_t}$
%  \caption{Randomized Pairwise FW} \label{algo:RPWFW}
%\end{algorithm}
%We however do not provide theoretical convergence guarantee for this randomized version, the proof being essentially of the same nature.

%\paragraph{Infinite Atomic set.} Algorithm \ref{algo:Randomized_away_general} consider a finite atomic set $\mathcal{A}$ and convergence analysis holds in such case. Though one can perfectly define a randomized version of AFW when the atomic set is infinite with a random set satisfying the same requirements as in Algo \ref{algo:Randomized_FW_general}.
%\begin{algorithm}[h]
%  \dots as in Algorithm \ref{algo:Randomized_away_general}, replacing line 1:
%  Choose $\mathcal{A}_t$ such that $\mathcal{P}(\vv\!\in\!\mathcal{A}_t)\!=\!\eta$ for all $\vv \in \mathcal{A}$
%  \caption{RAFW with infinite $\mathcal{A}$} \label{algo:RAFW_infinite_atomic_set}
%\end{algorithm}
%The randomized LMO of Line \ref{line:rafw_subsampled_lmo} is then similarly performed on the union of this $\mathcal{A}_t$ and $\mathcal{S}_t$, the support of $\xx_t$.

%\paragraph{Interaction Selection.}
%Cite it as an example of importance for which the objective is only generally strongly convex.

%Say that it is relevant to use FW in that case as it as another approach for doing structured matrix interaction and that it takes another approach than screening rules (which requires to keep in memory the sampling pattern?)

%\paragraph{Other polytope} Explore other polytope where the randomized LMO can be of interest not only it term of computing the number of gradient coefficients...







\section{Technical issues of previous work}\label{s:appendix_incomplete_frandi}

In this section we highlight some technical issues present in previous work.

\subsection{Randomized Frank-Wolfe in \citet{Frandi2016}}

\citet{Frandi2016} present a Randomized FW algorithm for the case of the $\ell_1$ ball in $\mathbb{R}^d$. Denote by $\mathcal{A}=\{\pm \boldsymbol{e}_i~~\forall i\in [d]\}$, where $\boldsymbol{e}_i$ is the canonical basis (i.e., the vector that is zero everywhere except on the $i$-th coordinate, where it equals one) the extremes atoms of the $\ell_1$ ball. Up to the iterative explicit implementation of the \textit{residuals}, \citep[Algorithm 2]{Frandi2016} with the sampling size $p\in[n]$ and our RFW (Algorithm \ref{algo:Randomized_FW_general}) are equivalent for the following choice of $\mathcal{A}_t$ in RFW
\begin{equation}
\mathcal{A}_t=\{\pm e_i~~\forall i\in \mathcal{I}_p\}~,~\text{ where $\mathcal{I}_p$ is random subset of $[d]$ of size $p$.}
\end{equation}


\paragraph{Convergence result.}
In this case, \citep[Proposition 2]{Frandi2016} gives the following convergence bound in expectation after $t$ iterations: 
\begin{eqnarray}\label{eq:expectation_rate_False}
\mathbb{E}(f(\xx_{t}))-f(\xx^*)\leq \frac{4 C_f}{t+2}~.
\end{eqnarray}
First, it is rather surprising that, unlike in our Theorem~\ref{th:expectation_rate}, the sub-sampling size $p$ does not appear the convergence bound. A closer inspection at their Lemma $2$ reveals some errors in their proof. For the remainder of this section we will use the notation in \citep{Frandi2016}.


% The aim of \citep[Lemma 2]{Frandi2016} is to prove \citep[equation (23)]{Frandi2016}
% \begin{eqnarray*}
% h_{k+1}=\mathbb{E}_{\mathcal{S}^{(k)}}\big[ h(\alpha_{\lambda}^{(k+1)})\big]\leq h_k-\lambda g_k +\lambda^2 C_f~.
% \end{eqnarray*}
% This is akin to the descent lemma in proof of first order algorithms. It is the same building block that is founded in most of the proofs of FW related algorithms. Similarly we have \eqref{eq:diff_with_frandi} with a factor $\eta=\frac{p}{d}$, that represents the cost of sub-sampling.

\paragraph{A problematic implication.} The proof of their Proposition 2 start with the following inequality derived from the curvature constant:
\begin{equation}
    f(\alpha_{\lambda}^{(k+1)})\leq f(\alpha^{(k)}) +\lambda \big(u^{(k)}-\alpha^{(k)}\big)^T\nabla f(\alpha^{(k)})+\lambda^2 C_f~.
\end{equation}
Then it is claimed that the following equation, Eq. (24) in their paper, is a direct consequence ``after some algebraic manipulations''
\begin{equation}\label{eq:frandi_problematic_equation}
\mathbb{E}_{\mathcal{S}^{(k)}}\big[f(\alpha_{\lambda}^{(k+1)})\big]\leq f(\alpha^{(k)}) +\lambda \mathbb{E}_{\mathcal{S}^{(k)}}\big[\big(u^{(k)}-\alpha^{(k)}\big)^T\widetilde\nabla_{\mathcal{S}^{(k)}} f(\alpha^{(k)})\big]+\lambda^2 C_f~.
\end{equation}
which is not clear unless $u^{(k)}$ is independent of the sampling set, something that is not verified given that it is chosen \emph{precisely  from} the sampling set.

\paragraph{Technical details.}
$\lambda$ being positive, for Eq.~\eqref{eq:frandi_problematic_equation} to be true, we should necessarily have the following
\begin{eqnarray}\label{eq:false_equation}
\mathbb{E}_{\mathcal{S}^{(k)}}\big[\big(u^{(k)}-\alpha^{(k)}\big)^T\nabla f(\alpha^{(k)})\big] \leq  \mathbb{E}_{\mathcal{S}^{(k)}}\big[\big(u^{(k)}-\alpha^{(k)}\big)^T\widetilde\nabla_{\mathcal{S}^{(k)}} f(\alpha^{(k)})\big]~.
\end{eqnarray}
$\alpha^{(k)}$ as well as $\nabla f(\alpha^{(k)})$ are deterministic with respect to the $\mathcal{S}^{(k)}$ sampling set so the previous equation is equivalent to
\begin{equation}
\mathbb{E}_{\mathcal{S}^{(k)}}\big[\big(u^{(k)}\big)^T\nabla f(\alpha^{(k)})\big]-\big(\alpha^{(k)}\big)^T\nabla f(\alpha^{(k)}) \leq  \mathbb{E}_{\mathcal{S}^{(k)}}\big[\big(u^{(k)}\big)^T\widetilde\nabla_{\mathcal{S}^{(k)}} f(\alpha^{(k)})\big] -\big(\alpha^{(k)}\big)^T\mathbb{E}_{\mathcal{S}^{(k)}}\big[\widetilde\nabla_{\mathcal{S}^{(k)}} f(\alpha^{(k)})\big]
\end{equation}
Since the sub-sampling of $\mathcal{S}^{(k)}$ being uniform and by definition of $\widetilde\nabla_{\mathcal{S}^{(k)}} f(\alpha^{(k)})$ in \citep[equation (14)]{Frandi2016} we have $\mathbb{E}_{\mathcal{S}^{(k)}}\big[\widetilde\nabla_{\mathcal{S}^{(k)}} f(\alpha^{(k)})\big]=\nabla f(\alpha^{(k)})$. Then \eqref{eq:false_equation} is equivalent to
\begin{eqnarray}
\mathbb{E}_{\mathcal{S}^{(k)}}\big[\big(u^{(k)}\big)^T\nabla f(\alpha^{(k)})\big] &\leq&  \mathbb{E}_{\mathcal{S}^{(k)}}\big[\big(u^{(k)}\big)^T\widetilde\nabla_{\mathcal{S}^{(k)}} f(\alpha^{(k)})\big]~.
\end{eqnarray}
Also by definition in \citep[equation (22)]{Frandi2016}, $u^{(k)}$ the FW atom has its support on $\mathcal{S}^{(k)}$ as well as from \citep[equation (6)]{Frandi2016} we have that $\big(u^{(k)}\big)^T\nabla f(\alpha^{(k)})<0$ . So that $\big(u^{(k)}\big)^T\nabla f(\alpha^{(k)})=\big(u^{(k)}\big)^T\nabla_{\mathcal{S}^{(k)}} f(\alpha^{(k)})$ and finally \eqref{eq:false_equation} is equivalent to
\begin{eqnarray}
\frac{|\mathcal{S}^{(k)}|}{p}\mathbb{E}_{\mathcal{S}^{(k)}}\big[\big(u^{(k)}\big)^T\widetilde\nabla_{\mathcal{S}^{(k)}} f(\alpha^{(k)})\big] &\leq&  \mathbb{E}_{\mathcal{S}^{(k)}}\big[\big(u^{(k)}\big)^T\widetilde\nabla_{\mathcal{S}^{(k)}} f(\alpha^{(k)})\big]~,
\end{eqnarray}
this last inequality being false in general because $\frac{|\mathcal{S}^{(k)}|}{p}<1$ and $\mathbb{E}_{\mathcal{S}^{(k)}}\big[\big(u^{(k)}\big)^T\widetilde\nabla_{\mathcal{S}^{(k)}} f(\alpha^{(k)})\big]\leq 0$.


%Denoting by $r_k=\nabla f(\alpha^{(k)})$ and $\tilde{r}_k=\tilde{\nabla}_{S^{(k)}} f(\alpha^{(k)})$, in their notation, it requires the following to be true:
%\begin{eqnarray*}
%E_k \left((u^{(k)}-\alpha^{(k)})^T r_k\right)&\leq & E_k \left((u^{(k)}-\alpha^{(k)})^T \tilde{r}_k\right)\\
%\Leftrightarrow E_k \left((u^{(k)}-\alpha^{(k)})^T r_k\right)&\leq & E_k \left((u^{(k)})^T \tilde{r}_k \right) - (\alpha^{(k)})^T r_k\\
%\Leftrightarrow  E_k \left((u^{(k)})^T r_t\right)&\leq & E_k \left((u^{(k)})^T \tilde{r}_t\right)
%\end{eqnarray*}
%Since $u^{(k)}$ is an atom of the $\ell_1$ ball, we have $(u^{(k)})^T r_t= \frac{S^{(k)}}{p}(u^{(k)})^T \tilde{r}_t$ and finally we should have the following inequality:
%\begin{eqnarray}\label{eq:last_proof_Randi_False}
%\frac{S^{(k)}}{p} E_k \left( (u^{(k)})^T \tilde{r}_t \right) \leq  E_k \left((u^{(k)})^T \tilde{r}_t\right).
%\end{eqnarray}
%The definition of $u^{(k)}$ satisfies:
%\begin{eqnarray}
%u^{(k)}=\underset{u\in \mathcal{V}}{\argmin } ~~ u^T \tilde{r}_t
%\end{eqnarray}
%where $\mathcal{V}$ is the set of extreme points of the $\ell_1$ ball. Its symmetry ensures that  $(u^{(k)})^T \tilde{r}_t$ is negative. Equation (\ref{eq:last_proof_Randi_False}) is then false.
